# Supplementary material for: Electron-phonon interaction and longitudinal-transverse phonon splitting in doped semiconductors
Source: arXiv:2202.02835 source file (2025-06-07)
Supplement: Supplementary file 1 [file SI_to_3d_material_PRL.pdf]

# SI to 'Fröhlich electron-phonon interaction and LO-TO splitting in doped semiconductors'

Francesco Macheda,[1] Paolo Barone,[2] and Francesco Mauri[3,1]

[1]*Istituto Italiano di Tecnologia, Graphene Labs, Via Morego 30, I-16163 Genova, Italy*

[2]*CNR-SPIN, Area della Ricerca di Tor Vergata, Via del Fosso del Cavaliere 100, I-00133 Rome, Italy*

[3]*Dipartimento di Fisica, Università di Roma La Sapienza, Roma, Italy*

## INTRODUCTION

In this supplementary material we give the derivations of the formulas used in the main text, beside giving more detailed computational information about the calculations that have been performed for this work. We also go deeper in some details whose proof was postponed.

In the section 'Definitions' we give a formal definition of all the quantities introduced in the main text, with a particular focus on the conventions used in this work. In the section 'Derivation of the asymptotic formulae for the LRCs' we start from the many body expression for the dynamical matrix and of the EPI and demonstrate that they can be rewritten in terms of quantities that correspond to the effective charges $Z_{s,\alpha}(\mathbf{q})$ and $\bar{Z}_{s,\alpha}(\mathbf{q})$ introduced in the main text; notice that these quantities have one atomic index and *only one cartesian index* (rank-1 tensors), instead of two as in the case of the Born effective charges (rank-2 tensors), and they contain the full charge response of a system to an external perturbation. In "Detailed computational information" we list all the *ab-initio* procedures used in this work, alongside with the parameters implemented. The last sections are instead devoted to practical consideration regarding the 'Dynamical quadrupoles', the 'Fermi energy shift', the 'Validity of the approximations to dielectric screening' used in the main text and to an analysis of the 'Unscreened charge density in the undoped case'.

## DEFINITIONS

We start from the definition of the problem writing down the Hamiltonian of the Khon-Sham system in presence of an external potential:

$$\hat{H} = \hat{T} + \hat{V}^{\mathrm{KS}} + \delta\hat{V}^{\mathrm{ext}}_{s,\alpha} \tag{1}$$

where $\hat{T}$ is the kinetic energy term, $\hat{V}^{\mathrm{KS}}$ is the self-consistent Khon-Sham potential including the electron-nuclei interaction (with the nuclei clamped in their equilibrium position), the Hartree and exchange-correlation terms; $\delta\hat{V}^{\mathrm{ext}}_{s,\alpha}$ is the external potential that is generated when the atoms of species $s$ are displaced along the direction $\alpha$. In this framework, the electron-phonon interaction is deduced deriving the expectation value of the Hamiltonian on the ground state with respect to the atomic displacement.

In general, for the monochromatic linear response problem we may write the atomic displacement as [1] $\upsilon_{s,\alpha}(\mathbf{q}) = \sum_p \lambda_\alpha e^{i\mathbf{q}\cdot(\mathbf{R}_p+\boldsymbol{\tau}_s)}$ where $\boldsymbol{\lambda}$ is the dimensional amplitude of the atomic displacement. For a generic charge density or potential $f$ that depends on the set of atomic positions $\{\mathbf{R}_p+\boldsymbol{\tau}_s\}$, we define its variation in the linear response regime with respect to the external perturbation $\upsilon_{s,\alpha}(\mathbf{q})$ as

$$\frac{\partial f(\mathbf{r},\{\mathbf{R}_p+\boldsymbol{\tau}_s\})}{\partial \lambda_\alpha}\Big|_{\lambda_\alpha=0} := \sum_{\mathbf{G}} \delta f_{s,\alpha}(\mathbf{q}+\mathbf{G},\{\mathbf{R}_p+\boldsymbol{\tau}_s\}) e^{i(\mathbf{q}+\mathbf{G})\cdot\mathbf{r}}, \tag{2}$$

where $\mathbf{G}$ are reciprocal lattice vectors. We will abbreviate $\frac{\partial f(\mathbf{r},\{\mathbf{R}_p+\boldsymbol{\tau}_s\})}{\partial \lambda_\alpha}\Big|_{\lambda_\alpha=0} := \frac{\partial f(\mathbf{r},\{\mathbf{R}_p+\boldsymbol{\tau}_s\})}{\partial \lambda_\alpha}$; $\sum_{\mathbf{G}} \delta f_{s,\alpha}(\mathbf{q}+\mathbf{G},\{\mathbf{R}_p+\boldsymbol{\tau}_s\}) e^{i\mathbf{G}\cdot\mathbf{r}}$ is a cell-periodic function and, using a notation similar to the one of Ref. [2], may be as well indicated with $\delta f^{\mathbf{q}}_{s,\alpha}(\mathbf{r})$; clearly, we have also that $\delta f_{s,\alpha}(\mathbf{q},\{\mathbf{R}_p+\boldsymbol{\tau}_s\}) = \frac{1}{V}\int d\mathbf{r} f^{\mathbf{q}}_{s,\alpha}(\mathbf{r})$.

With the above definitions, we now consider a choice of the unit cell (primed quantities) where the atomic positions inside the unit cell are shifted by a certain constant vector $\mathbf{a}$, such that $\boldsymbol{\tau}'_s = \boldsymbol{\tau}_s + \mathbf{a}$; in this case we notice that $\upsilon'_{s,\alpha}(\mathbf{q}) = \upsilon_{s,\alpha}(\mathbf{q}) e^{i\mathbf{q}\cdot\mathbf{a}}$, having defined $\boldsymbol{\lambda}' = \boldsymbol{\lambda} e^{-i\mathbf{q}\cdot\mathbf{a}}$—this new definition of the dimensional amplitude follows from the fact that in principle following a translation we should send $\mathbf{R}'_p \rightarrow \mathbf{R}_p + \mathbf{a}$, but we can avoid to do so if we modulate also the dimensional displacement amplitude. For the electronic coordinates, the reference frame change corresponds to a shift of the form $\mathbf{r}' = \mathbf{r} + \mathbf{a}$; the response to a monochromatic perturbation of wavevector $\mathbf{q}$ is written as $\frac{\partial f'(\mathbf{r}',\{\mathbf{R}_p+\boldsymbol{\tau}'_s\})}{\partial \lambda'_\alpha} = \delta f'^{\mathbf{q}}_{s,\alpha}(\mathbf{r}') e^{i\mathbf{q}\cdot\mathbf{r}'} = \frac{\partial f(\mathbf{r},\{\mathbf{R}_p+\boldsymbol{\tau}_s\})}{\partial \lambda_\alpha} e^{i\mathbf{q}\cdot\mathbf{a}} = \delta f^{\mathbf{q}}_{s,\alpha}(\mathbf{r}) e^{i\mathbf{q}\cdot\mathbf{r}'}$ which means that $\delta f'^{\mathbf{q}}_{s,\alpha}(\mathbf{r}') = \delta f^{\mathbf{q}}_{s,\alpha}(\mathbf{r})$, i. e. that the response to a monochromatic perturbation behaves as a scalar, and this nice property follows from the form of the atomic displacement chosen in this work. In other conventions, the transformations laws are different.

The derivation of the LRCs is properly obtained as a function of the above defined charge density and potential change instead of the effective charges, which are nonetheless univocally determined via the charge density change, as we will see later in details. We anticipate that the connection is straightforward and can be performed, computing the macroscopical total *unscreened* charge density change, $\delta\bar{\rho}^{\text{tot}}_{s,\alpha}(\mathbf{q})$, produced by $\upsilon_{s,\alpha}(\mathbf{q})$, via the relation

$$\bar{Z}_{s,\alpha}(\mathbf{q}) = i\frac{V}{eq}\delta\bar{\rho}^{\text{tot}}_{s,\alpha}(\mathbf{q}). \tag{3}$$

Actually, this is the *operative* way that we use in this work in order to deduce the effective charges from first-principle calculations, i.e. we compute the total charge density change for each monochromatic perturbation of wavevector $\mathbf{q}$ of the external perturbation and then deduce the effective charges. In agreement with the phase choice operated for the atomic displacements, we also define the Fourier transform between the force constant and the dynamical matrix to be

$$C_{ss'}(\mathbf{q}) \propto \sum_p C_{ss'}(\mathbf{R}_p) e^{i\mathbf{q}\cdot(\mathbf{R}_p+\boldsymbol{\tau}_s-\boldsymbol{\tau}_{s'})}. \tag{4}$$

Coherently, the phonon displacements are defined as

$$\boldsymbol{v}^{\nu}_{sp}(\mathbf{q}) := \mathbf{e}^{\nu}_s(\mathbf{q}) e^{i\mathbf{q}\cdot(\mathbf{R}_p+\boldsymbol{\tau}_s)} \tag{5}$$

while in other conventions (such as the one used in QUANTUM ESPRESSO) the phase factor dependent on the atomic position is missing. Similarly, the difference between Eq. 3 of the main text and Eq. 2 of Ref. [3] is due to this same reason.

## DERIVATION OF THE ASYMPTOTIC FORMULAE FOR THE LRCS

In this section we provide the derivation for the asymptotic formulae of the LRCs of the EPI and of the dynamical matrix. The derivation follows the logic of Refs. [4] and [1], but it is extended to the case of finite doping and temperature. To not overburden the notation, we will explicit the necessary $n$ and $T$ dependence only when strictly needed. We will work in an all-electron formalism, since the asymptotic formulas are the same in a pseudopotential approach—we will highlight the differences later when necessary. Moreover, we will work in the RPA approximation for simplicity, but since the conclusion on the *form* of the LRCs depends just on the long wavelength expansion of the inverse dielectric matrix, and this does not depend on the inclusion of exchange-correlation terms as long as we are dealing with local approximations [5], our derivation will be of general validity.

We introduce the following response matrix, as done in [1]:

$$\Xi(\mathbf{q}+\mathbf{G},\mathbf{q}+\mathbf{G}') = \frac{|\mathbf{q}+\mathbf{G}|^2}{4\pi}\epsilon(\mathbf{q}+\mathbf{G},\mathbf{q}+\mathbf{G}') = \frac{|\mathbf{q}+\mathbf{G}|^2}{4\pi}\delta_{\mathbf{G}\mathbf{G}'} - \chi^0(\mathbf{q}+\mathbf{G},\mathbf{q}+\mathbf{G}') \tag{6}$$

where $\mathbf{G},\mathbf{G}'$ are reciprocal lattice vectors and where the last equality holds only in the RPA approximation. Notice that here the $\epsilon$ matrix represents *dielectric* response. We can also

notice that $\Xi(\mathbf{q}+\mathbf{G},\mathbf{q}+\mathbf{G}')$ is Hermitian and analytic since $\chi^0(\mathbf{q}+\mathbf{G},\mathbf{q}+\mathbf{G}')$ has both properties [4]. We notice that the $\Xi$ matrix is involved in the writing of the 'Maxwell's equation'

$$\frac{|\mathbf{q}+\mathbf{G}|^2}{4\pi}\cdot\delta V^{\rm ext}_{s,\alpha}(\mathbf{q}+\mathbf{G})=\sum_{\mathbf{G}'}\Xi(\mathbf{q}+\mathbf{G},\mathbf{q}+\mathbf{G}')\delta V^{\rm tot}_{s,\alpha}(\mathbf{q}+\mathbf{G}')=\delta\rho^{\rm ext}_{s,\alpha}(\mathbf{q}+\mathbf{G}) \qquad (7)$$

where $\delta V^{\rm tot}_{s,\alpha}(\mathbf{q}+\mathbf{G})$ is the change of the total potential produced by an external charge perturbation $\delta\rho^{\rm ext}_{s,\alpha}(\mathbf{q}+\mathbf{G})$ generated by $\upsilon_{s,\alpha}(\mathbf{q})$. Given that the ionic charge may be written as a function of the atomic charges $Z_s$ as $\rho^{\rm ion}(\mathbf{r})=\sum_{ps}Z_s e\delta(\mathbf{r}-\mathbf{R}_p-\boldsymbol{\tau}_s)$, we then identify $\frac{\partial\rho^{\rm ion}(\mathbf{r})}{\partial\lambda_\alpha}=\delta\rho^{\rm ext}_{s,\alpha}(\mathbf{q}+\mathbf{G})e^{i\mathbf{q}\cdot\mathbf{r}}$. It follows that

$$\delta\rho^{\rm ext}_{s,\alpha}(\mathbf{q}+\mathbf{G})=-i\frac{Z_s e}{V}\left[(q_\alpha+G_\alpha)e^{-i\mathbf{G}\cdot\boldsymbol{\tau}_s}\right]. \qquad (8)$$

An equation analogous to Eq. 6 may be written for the $\Xi^{-1}$ matrix as

$$\Xi^{-1}(\mathbf{q}+\mathbf{G},\mathbf{q}+\mathbf{G}')=\frac{4\pi}{|\mathbf{q}+\mathbf{G}'|^2}\epsilon^{-1}(\mathbf{q}+\mathbf{G},\mathbf{q}+\mathbf{G}'); \qquad (9)$$

since the appearance of LRC is connected to the inversion of the $\Xi$ matrix, we start analyzing this inversion procedure.

**Inversion of $\Xi$**

Following [1, 4] we write:

$$\Xi=\begin{pmatrix}P & Q\\ Q^\dagger & S\end{pmatrix}, \qquad (10)$$

$$\Xi^{-1}=\begin{pmatrix}W & X\\ X^\dagger & Z\end{pmatrix}, \qquad (11)$$

where $P=\Xi(\mathbf{q},\mathbf{q})$ is called the 'head' of the matrix, $Q=\Xi(\mathbf{q},\mathbf{q}+\mathbf{G}')$ is the 'wing' and $S=\Xi(\mathbf{q}+\mathbf{G},\mathbf{q}+\mathbf{G}')$ is the 'body', and the same goes for $W,X,Z$. We can symbolically relate the elements of the two matrices with the following relations:

$$W=(P-QS^{-1}Q^\dagger)^{-1}, \qquad (12)$$

$$X=-WQS^{-1}, \qquad (13)$$

$$Z=S^{-1}+X^\dagger W^{-1}X. \qquad (14)$$

$\Xi^{-1}$ may then be rewritten as:

$$\Xi^{-1} = \begin{pmatrix} W & X \\ X^{\dagger} & S^{-1} + X^{\dagger} W^{-1} X \end{pmatrix}. \tag{15}$$

For what will be evident later, we define:

$$\hat{\Xi}^{-1} = \begin{pmatrix} W & X \\ X^{\dagger} & X^{\dagger} W^{-1} X \end{pmatrix}, \tag{16}$$

which can be rewritten as

$$\hat{\Xi}^{-1}(\mathbf{q}+\mathbf{G},\mathbf{q}+\mathbf{G}') = \frac{\hat{\Xi}^{-1}(\mathbf{q},\mathbf{q}+\mathbf{G}')\hat{\Xi}^{-1}(\mathbf{q}+\mathbf{G},\mathbf{q})}{\hat{\Xi}^{-1}(\mathbf{q},\mathbf{q})} = \frac{\hat{\Xi}^{-1}(\mathbf{q},\mathbf{q}+\mathbf{G}')\hat{\Xi}^{-1,\mathrm{c.c.}}(\mathbf{q},\mathbf{q}+\mathbf{G})}{\hat{\Xi}^{-1}(\mathbf{q},\mathbf{q})}.$$

Since we will be interested in the asymptotic limits of the above expression, and $\Xi$ depends on $\chi^0$, it is necessary to study the asymptotic behaviour of the independent particle polarizability in semiconductors, which is matter of the next section.

### Independent particle polarizability limits

The expression for the independent particle polarizability is:

$$\chi^0(\mathbf{q}+\mathbf{G},\mathbf{q}+\mathbf{G}') = \frac{2}{V}\sum_{mm'\mathbf{k}} \frac{f_{m\mathbf{k}} - f_{m'\mathbf{k}+\mathbf{q}}}{\epsilon_{m\mathbf{k}} - \epsilon_{m'\mathbf{k}+\mathbf{q}}} \int d\mathbf{r} u_{m\mathbf{k}}(\mathbf{r}) u^{\mathrm{c.c}}_{m'\mathbf{k}+\mathbf{q}+\mathbf{G}}(\mathbf{r}) \int d\mathbf{r}' u^{\mathrm{c.c}}_{m\mathbf{k}}(\mathbf{r}') u_{m'\mathbf{k}+\mathbf{q}+\mathbf{G}'}(\mathbf{r}') \tag{17}$$

where the factor 2 comes from spin degeneracy. For undoped semiconductors at 0K we can write

$$\lim_{\mathbf{q}\to\mathbf{0}} \chi^0(\mathbf{q},\mathbf{q}) = \frac{2q_\alpha q_\beta}{V}\sum_{mn\mathbf{k}} \frac{\theta(\epsilon_{n\mathbf{k}}) - \theta(\epsilon_{m\mathbf{k}})}{\epsilon_{m\mathbf{k}} - \epsilon_{n\mathbf{k}}} \langle u_{m\mathbf{k}} | \partial_{\mathbf{k}_\alpha} u_{n\mathbf{k}} \rangle^* \langle u_{m\mathbf{k}} | \partial_{\mathbf{k}_\beta} u_{n\mathbf{k}} \rangle \coloneqq \mathbf{q} \cdot B \cdot \mathbf{q} \tag{18}$$

$$\lim_{\mathbf{q}\to\mathbf{0}} \chi^0(\mathbf{q},\mathbf{q}+\mathbf{G}') = \frac{2q_\alpha}{V}\sum_{mn\mathbf{k}} \frac{\theta(\epsilon_{n\mathbf{k}}) - \theta(\epsilon_{m\mathbf{k}})}{\epsilon_{m\mathbf{k}} - \epsilon_{n\mathbf{k}}} \langle u_{m\mathbf{k}} | \partial_{\mathbf{k}_\alpha} u_{n\mathbf{k}} \rangle^{\mathrm{c.c}} \langle u_{m\mathbf{k}} | u_{n\mathbf{k}+\mathbf{G}'} \rangle \coloneqq \mathbf{q} \cdot \mathbf{A}(\mathbf{G}') + O(q^2) \tag{19}$$

$$\lim_{\mathbf{q}\to\mathbf{0}} \chi^0(\mathbf{q}+\mathbf{G},\mathbf{q}+\mathbf{G}') = \frac{2}{V}\sum_{mn\mathbf{k}} \frac{\theta(\epsilon_{n\mathbf{k}}) - \theta(\epsilon_{m\mathbf{k}})}{\epsilon_{m\mathbf{k}} - \epsilon_{n\mathbf{k}}} \langle u_{m\mathbf{k}} | u_{n\mathbf{k}+\mathbf{G}} \rangle^{\mathrm{c.c}} \langle u_{m\mathbf{k}} | u_{n\mathbf{k}+\mathbf{G}'} \rangle, \tag{20}$$

where $\theta$ is the Heaviside function, we have used that $\langle u_{v\mathbf{k}}|u_{c\mathbf{k}}\rangle = 0$ ($v$ stands for 'valence' and $c$ for 'conduction') and that there are no intraband transitions that can cause the energy denominator to vanish so that we can safely replace $\epsilon_{m\mathbf{k}+\mathbf{q}} \to \epsilon_{m\mathbf{k}}$, and we have defined $|u_{\mathbf{k}+\mathbf{G}}\rangle = e^{-i\mathbf{G}\cdot\mathbf{r}}|u_{\mathbf{k}}\rangle$. The above expressions for $\chi^0$ are reflected on the asymptotic limits of $\Xi^{-1}$ in the following way:

$$\begin{cases} \lim_{\mathbf{q}\to 0} \Xi^{-1}(\mathbf{q}+\mathbf{G},\mathbf{q}+\mathbf{G}') = S^{-1}(\mathbf{G},\mathbf{G}') + \sum_{\mathbf{G}\mathbf{G}'} \frac{\mathbf{q}\cdot\mathbf{A}'(\mathbf{G})}{\mathbf{q}\cdot B'\cdot\mathbf{q}} S^{-1}(\mathbf{G},\mathbf{G}') \frac{\mathbf{q}\cdot\mathbf{A}'^{c.c}(\mathbf{G}')}{\mathbf{q}\cdot B'\cdot\mathbf{q}} & \mathbf{G}\neq 0 \wedge \mathbf{G}'\neq 0 \\ \lim_{\mathbf{q}\to 0} \Xi^{-1}(\mathbf{q},\mathbf{q}+\mathbf{G}') = \frac{\mathbf{q}\cdot\mathbf{A}'(\mathbf{G}')}{\mathbf{q}\cdot B'\cdot\mathbf{q}} \quad \mathbf{G}'\neq 0 \\ \lim_{\mathbf{q}\to 0} \Xi^{-1}(\mathbf{q}+\mathbf{G},\mathbf{q}) = \frac{\mathbf{q}\cdot\mathbf{A}'^{c.c}(\mathbf{G})}{\mathbf{q}\cdot B'\cdot\mathbf{q}} \quad \mathbf{G}\neq 0 \\ \lim_{\mathbf{q}\to 0} \Xi^{-1}(\mathbf{q},\mathbf{q}) = \frac{1}{\mathbf{q}\cdot B'\cdot\mathbf{q}} \end{cases} \tag{21}$$

where $\mathbf{A}'(\mathbf{G})$ and $B'$ are system dependent quantities. In particular, the expression for $\mathbf{A}'$—which will be used in the following— is

$$\mathbf{A}'(\mathbf{G}) = \sum_{\mathbf{G}'\neq 0} \mathbf{A}(\mathbf{G}')S^{-1}(\mathbf{G}',\mathbf{G}). \tag{22}$$

From the above asymptotic formula for the $\Xi^{-1}$ matrix we notice that all the long range components stem from the $\hat{\Xi}^{-1}$ matrix.

For doped semiconductors the intraband term will modify the above expression in the regime of metallization of the response, since the limits of the intraband contribution to the independent particle polarizability are

$$\lim_{\mathbf{q}\to\mathbf{0}} \chi^0(\mathbf{q},\mathbf{q}) = \frac{2}{V}\sum_{m\mathbf{k}} \frac{f_{m\mathbf{k}} - f_{m\mathbf{k}+\mathbf{q}}}{\epsilon_{m\mathbf{k}} - \epsilon_{m\mathbf{k}+\mathbf{q}}} \tag{23}$$

$$\lim_{\mathbf{q}\to\mathbf{0}} \chi^0(\mathbf{q},\mathbf{q}+\mathbf{G}') = \frac{2}{V}\sum_{m\mathbf{k}} \frac{f_{m\mathbf{k}} - f_{m\mathbf{k}+\mathbf{q}}}{\epsilon_{m\mathbf{k}} - \epsilon_{m\mathbf{k}+\mathbf{q}}} \langle u_{m\mathbf{k}}|u_{m\mathbf{k}+\mathbf{G}'}\rangle \tag{24}$$

$$\lim_{\mathbf{q}\to\mathbf{0}} \chi^0(\mathbf{q}+\mathbf{G},\mathbf{q}+\mathbf{G}') = \frac{2}{V}\sum_{mm'\mathbf{k}} \frac{f_{m\mathbf{k}} - f_{m'\mathbf{k}+\mathbf{q}}}{\epsilon_{m\mathbf{k}} - \epsilon_{m'\mathbf{k}+\mathbf{q}}} \langle u_{m\mathbf{k}}|u_{m'\mathbf{k}+\mathbf{G}}\rangle^{c.c} \langle u_{m\mathbf{k}}|u_{m'\mathbf{k}+\mathbf{G}'}\rangle, \tag{25}$$

where $m, m'$ are energy levels which are near the Fermi energy and we have used the orthonormalization relation $\langle u_{m\mathbf{k}}|u_{m'\mathbf{k}}\rangle = \delta_{mm'}$. The limits for $\Xi^{-1}$ will change accordingly, being regularized in an energy region around the Fermi level, as explained in the main text of the article. Also, we will show in the following sections how the asymptotic expression of the total charge change are modified in presence of doping.

**LRC of the dynamical matrix**

The microscopic expression of the part of the dynamical matrix that gives rise to LRCs can be written as [4]

$$C_{ss',\alpha\beta}(\mathbf{q}) = \frac{4\pi Z_s Z_{s'} e^2}{V} \sum_{\mathbf{G}\mathbf{G}'} \epsilon^{-1}(\mathbf{q}+\mathbf{G},\mathbf{q}+\mathbf{G}') \frac{4\pi}{|\mathbf{q}+\mathbf{G}'|^2} (q_\alpha + G_\alpha)(q_\beta + G'_\beta) e^{i(\mathbf{G}\cdot\boldsymbol{\tau}_s - \mathbf{G}'\cdot\boldsymbol{\tau}_{s'})} = \frac{Z_s Z_{s'} e^2}{V} \sum_{\mathbf{G}\mathbf{G}'} \Xi^{-1}(\mathbf{q}+\mathbf{G},\mathbf{q}+\mathbf{G}')(q_\alpha + G_\alpha)(q_\beta + G'_\beta) e^{i(\mathbf{G}\cdot\boldsymbol{\tau}_s - \mathbf{G}'\cdot\boldsymbol{\tau}_{s'})}. \tag{26}$$

For completeness, we report that the total dynamical matrix $C^{tot}$ can be expressed as a function of the above contribution as [4]

$$C^{\mathrm{tot}}_{ss',\alpha\beta}(\mathbf{q}) = C_{ss',\alpha\beta}(\mathbf{q}) - \delta_{ss'} \sum_{s''} C_{ss'',\alpha\beta}(\mathbf{0}), \tag{27}$$

where the second term is needed to enforce the translational invariance, from which effective charge neutrality follows [4].

As explained in the previous sections, all the long range components of the $\Xi^{-1}$ matrix come from $\hat{\Xi}^{-1}$, so that we can isolate the long range component of the dynamical matrix writing

$$C^{\mathrm{L}}_{ss',\alpha\beta}(\mathbf{q}) = \frac{Z_s Z_{s'} e^2}{V} \sum_{\mathbf{G},\mathbf{G}'} \frac{\hat{\Xi}^{-1}(\mathbf{q},\mathbf{q}+\mathbf{G}')\hat{\Xi}^{-1,\mathrm{c.c.}}(\mathbf{q},\mathbf{q}+\mathbf{G})}{\hat{\Xi}^{-1}(\mathbf{q},\mathbf{q})} (q_\alpha + G_\alpha)(q_\beta + G'_\beta) e^{i(\mathbf{G}\cdot\boldsymbol{\tau}_s - \mathbf{G}'\cdot\boldsymbol{\tau}_{s'})}. \tag{28}$$

We define

$$\delta\phi_{s,\alpha}(\mathbf{q}) = -i\frac{Z_s e}{V} \sum_{\mathbf{G}'} \hat{\Xi}^{-1}(\mathbf{q},\mathbf{q}+\mathbf{G}')(q_\alpha + G'_\alpha) e^{-i\mathbf{G}'\cdot\boldsymbol{\tau}_s} = \sum_{\mathbf{G}'} \hat{\Xi}^{-1}(\mathbf{q},\mathbf{q}+\mathbf{G}')\delta\rho^{\mathrm{ext}}_{s,\alpha}(\mathbf{q}+\mathbf{G}'), \tag{29}$$

where we have used Eq. 8 for the last equality. $\delta\phi_{s,\alpha}(\mathbf{q})$ is interpreted, in light of Eq. 7, as the total *macroscopic* potential change generated by the external charge perturbation. In fact, the short range component of $\Xi^{-1}$, i.e. $(\Xi^{-1} - \hat{\Xi}^{-1})$, has null head and wings and therefore $\hat{\Xi}^{-1}(\mathbf{q},\mathbf{q}+\mathbf{G}) = \Xi^{-1}(\mathbf{q},\mathbf{q}+\mathbf{G})$—in other words $(\Xi^{-1} - \hat{\Xi}^{-1})$ cannot create additional macroscopic potentials and therefore $\delta\phi_{s',\beta}(\mathbf{q})$ is directly the total change of the macroscopic potential. The LRC may be now written as

$$C^{\mathrm{L}}_{ss',\alpha\beta}(\mathbf{q}) = \frac{V}{\hat{\Xi}^{-1}(\mathbf{q},\mathbf{q})} \delta\phi^{\mathrm{c.c.}}_{s,\alpha}(\mathbf{q})\delta\phi_{s',\beta}(\mathbf{q}) = V\hat{\Xi}^{-1}(\mathbf{q},\mathbf{q}) \frac{\delta\phi^{\mathrm{c.c.}}_{s,\alpha}(\mathbf{q})}{\hat{\Xi}^{-1}(\mathbf{q},\mathbf{q})} \frac{\delta\phi_{s',\beta}(\mathbf{q})}{\hat{\Xi}^{-1}(\mathbf{q},\mathbf{q})}, \tag{30}$$

where all the terms entering the above expression are all *macroscopic*. In particular, we can interpret $\delta\phi_{s',\beta}(\mathbf{q})/\hat{\Xi}^{-1}(\mathbf{q},\mathbf{q})$ as the total *unscreened macroscopic* change in charge density that is produced in the system as a consequence of the external perturbation. We will demonstrate this identification later.

**For the case of undoped semiconductors** we may use the asymptotic expression for the $\hat{\Xi}$ matrix, obtaining:

$$\lim_{\mathbf{q}\to 0}\frac{\delta\phi_{s',\beta}(\mathbf{q})}{\hat{\Xi}^{-1}(\mathbf{q},\mathbf{q})} = -i\lim_{\mathbf{q}\to 0}\left[q_\beta Z_{s'} + \sum_{\mathbf{G}'\neq 0}\mathbf{q}\cdot\mathbf{A}'(\mathbf{G}')(q_\beta + G'_\beta)Z_{s'}e^{-i\mathbf{G}'\cdot\boldsymbol{\tau}_{s'}}\right] =$$

$$-i\lim_{\mathbf{q}\to 0}\left[q_\beta Z_{s'} + \sum_{\mathbf{G}'\neq 0}\mathbf{q}\cdot\mathbf{A}'(\mathbf{G}')G'_\beta Z_{s'}e^{-i\mathbf{G}'\cdot\boldsymbol{\tau}_{s'}}\right]. \tag{31}$$

In general, the above expression thus admit a Taylor expansion of the form

$$\frac{\delta\phi_{s',\beta}(\mathbf{q})}{\hat{\Xi}^{-1}(\mathbf{q},\mathbf{q})} = \frac{e}{V}\sum_\gamma q_\gamma F_{s',\beta\gamma}(\mathbf{q}). \tag{32}$$

The $\mathbf{q}$ dependence of $F$ comes from the higher-order expansions of the wings of the polarizability matrix, that have not been explicitly written but can be easily be introduced in the calculation; the limit of equation 31 shows that we can expand

$$F_{s',\alpha\beta}(\mathbf{q}) = -iZ^*_{s',\alpha\beta} - \sum_\gamma \frac{1}{2}q_\gamma Q_{s',\alpha\beta\gamma} + \sum_{\gamma\delta} i q_\gamma q_\delta \frac{1}{6}O_{s',\alpha\beta\gamma\delta} + O(q^3) \tag{33}$$

where the various terms of the expansion can be identified with the Born effective charges, dynamical effective quadrupoles and so on [1]. We remind that the identification of the effective charges is legitimate only if the macroscopic electric field is zero, which is not the case for the above procedure. Nonetheless, we notice that the condition of zero macroscopic electric field can be obtained by solving the electrostatic problem with the imposition that $\delta V^{tot}_{s,\alpha}(\mathbf{q}) = 0$; in this case one obtains directly the unscreened quantity $F_{s',\beta\gamma}(\mathbf{q})$ from the total charge density. We now show in details how.

The imposition that $\delta V^{\rm tot}_{s,\alpha}(\mathbf{q}) = 0$ for each possible charge perturbation can be satisfied only if in Eq. 15 we have $W = \eta$ and $X = \eta$, where $\eta$ is an infinitesimal small number. We notice that $\lim_{\eta\to 0}\hat{\Xi}^{-1} = 0$, so that we are left only with the short range component of the $\Xi^{-1}$ matrix. The total potential may now be written, for $\mathbf{G}\neq 0$ as

$$\delta\bar{V}^{\rm tot}_{s,\alpha}(\mathbf{q}+\mathbf{G}) = \sum_{\mathbf{G}'\neq 0} S^{-1}(\mathbf{q}+\mathbf{G},\mathbf{q}+\mathbf{G}')\delta\rho^{\rm ext}_{s,\alpha}(\mathbf{q}+\mathbf{G}'). \tag{34}$$

where the bar indicates that the quantities are computed imposing $\delta V^{\rm tot}_{s,\alpha}(\mathbf{q}) = 0$. By the definition of $\chi^0$, i.e. the response function connecting the induced density to the change of total potential, we obtain

$$\delta\bar{\rho}^{\rm ind}_{s,\alpha}(\mathbf{q}) = \sum_{\substack{\mathbf{G}\neq 0\\ \mathbf{G}'\neq 0}} \chi^0(\mathbf{q},\mathbf{q}+\mathbf{G}) S^{-1}(\mathbf{q}+\mathbf{G},\mathbf{q}+\mathbf{G}')\delta\rho^{\rm ext}_{s,\alpha}(\mathbf{q}+\mathbf{G}'). \tag{35}$$

To obtain the total charge, $\delta\bar{\rho}^{\rm tot}_{s,\alpha}(\mathbf{q})$, in this particular setup, we sum $\delta\rho^{\rm ext}_{s,\alpha}(\mathbf{q})$ to $\delta\bar{\rho}^{\rm ind}_{s,\alpha}(\mathbf{q})$ and, expressing the wing of $\chi^0$ in its limit Eq. 19, we finally obtain exactly the r.s.h. of Eq. 31; this proves that when putting to zero the change of the macroscopic total potential in the electrostatic problem we obtain a total charge density change which we can expand exactly as that of Eqs. 32 and 33, i.e. $\delta\bar{\rho}^{\rm tot}_{s,\alpha}(\mathbf{q})$ is the unscreened effective charge density, equal to $\delta\phi_{s',\beta}(\mathbf{q})/\hat{\Xi}^{-1}(\mathbf{q},\mathbf{q})$. This also shows that $\hat{\Xi}^{-1}(\mathbf{q},\mathbf{q})\delta\bar{\rho}^{\rm tot}_{s,\alpha}(\mathbf{q}) = \delta\phi_{s',\beta}(\mathbf{q}) = 4\pi/q^2\delta\rho^{\rm tot}_{s,\alpha}(\mathbf{q})$ where we have used the RPA relation between potential and charge, identifying therefore $\delta\phi_{s',\beta}(\mathbf{q}) = \delta V^{\rm tot}_{s',\beta}(\mathbf{q})$, which finally bring us to $\delta\rho^{\rm tot}_{s,\alpha}(\mathbf{q}) = \epsilon^{-1}(\mathbf{q},\mathbf{q})\delta\bar{\rho}^{\rm tot}_{s,\alpha}(\mathbf{q})$ and justifies the use of the bar notation over the quantities computed with the imposition of null electrostatic potential at $\mathbf{G} = \mathbf{0}$.

Finally, the identification of the various terms of Eq. 33 with the effective charges can be done in line with Ref. [1]. For example, the Born effective charge of the atom $s$ is defined as

$$Z^*_{s,\alpha\beta} = \frac{V}{e}\frac{\partial P_\alpha}{\partial v_{s,\beta}(\mathbf{0})}\Big|_{\mathbf{E}=\mathbf{0}}, \tag{36}$$

where $P_\alpha$ is a Cartesian component of the polarization vector per unit volume, and which in our notation is equivalent to write

$$Z^*_{s,\alpha\beta} = \frac{V}{e}\frac{\partial P_\alpha}{\partial \lambda_\beta}\Big|_{\mathbf{q}=\mathbf{0},\mathbf{E}=\mathbf{0}}. \tag{37}$$

We now define the charge density change on a single atom (SA) exploiting the superposition of the charge density change in the linear regime for the response

$$\delta\bar{\rho}^{\rm SA}_{s,\beta}(\mathbf{r}-\mathbf{R}_p-\boldsymbol{\tau}_s) = \frac{V}{(2\pi)^3}\int d\mathbf{q}\,\delta\bar{\rho}^{\mathbf{q},\rm tot}_{s,\beta}(\mathbf{r})e^{-i\mathbf{q}\cdot(\mathbf{R}_p-\boldsymbol{\tau}_s-\mathbf{r})}, \tag{38}$$

with the inverse Fourier transform given by

$$\delta\bar{\rho}^{\mathbf{q},\rm tot}_{s,\beta}(\mathbf{r}) = \sum_p \delta\bar{\rho}^{\rm SA}_{s,\beta}(\mathbf{r}-\mathbf{R}_p-\boldsymbol{\tau}_s)e^{i\mathbf{q}\cdot(\mathbf{R}_p+\boldsymbol{\tau}_s-\mathbf{r})}. \tag{39}$$

Then, we write

$$\left.\frac{\partial P_\alpha}{\partial \lambda_\beta}\right|_{\mathbf{q}=\mathbf{0},\mathbf{E}=\mathbf{0}} = \frac{1}{NV}\sum_p \int_{crystal} d\mathbf{r}(r_\alpha - R_{p,\alpha} - \tau_{s,\alpha})\delta\bar{\rho}^{\mathrm{SA}}_{s,\beta}(\mathbf{r}-\mathbf{R}_p-\boldsymbol{\tau}_s) = \tag{40}$$

$$\frac{i}{NV}\int_{crystal} d\mathbf{r}\frac{\partial}{\partial q_\alpha}\delta\bar{\rho}^{\mathbf{q},\mathrm{tot}}_{s,\beta}(\mathbf{r}) = i\frac{\partial}{\partial q_\alpha}\delta\bar{\rho}^{\mathrm{tot}}_{s,\beta}(\mathbf{q})\Big|_{\mathbf{q}=0}. \tag{41}$$

The last equality proves the identification between effective charges and the expansion of the unscreened charge density change; the same can be done also for higher orders. Notice that, as mentioned in the introduction, thanks to the choice of the phase factor the expansion of the unscreened charge density change is independent on the choice of the basis vectors of the atomic positions. We now comment how the use of pseudopotentials impacts the formalism of this section. Pseudopotentials generally contain local and non-local parts; following a collective atomic displacement, the local part of the pseudopotential produces an external charge in a form similar Eq. 8, but which includes a form factor coming from the shape of the potential. In fact, one can write the ionic charges as $\rho^{\mathrm{ion}}(\mathbf{r}) = \sum_{ps} Z^v_s f_s(\mathbf{r}-\mathbf{R}_p-\boldsymbol{\tau}_s)$ where $Z^v_s$ is the valence pseudocharge and it holds that $\int_0^{r_c} dr f_s(r) = 1$, where $r_c$ is the core radius. Then, the change of the external charge density can be written as

$$\delta\rho^{\mathrm{ext}}_{s,\alpha}(\mathbf{q}+\mathbf{G}) = -i\frac{Z^v_s e}{V}\left[(q_\alpha+G_\alpha)f_s(\mathbf{q}+\mathbf{G})e^{-i\mathbf{G}\cdot\boldsymbol{\tau}_s}\right], \tag{42}$$

with $f_s(\mathbf{0}) = 1$. We suppose that using the form of the ionic charge density and of its change upon perturbation proper for the pseudonuclei has a negligible impact on the observable for $q > 1/r_c$. Similarly, the non-local part of the pseudopotential in principle produces a non-local charge density change for $r < r_c$, which cannot be described in our formalism—in particular, the identification of the matrix connecting the total potential to the charge with the dielectric one is no more correct. Again, we suppose that these effects have impact only for $q > 1/r_c$.

Following the above considerations, at the end we can recast the formula for the unscreened effective charges as

$$\bar{Z}_{s,\alpha} = \frac{iV}{eq}\sum_{\mathbf{G}'}\frac{\hat{\Xi}^{-1}(\mathbf{q},\mathbf{q}+\mathbf{G}')}{\hat{\Xi}^{-1}(\mathbf{q},\mathbf{q})}\delta\rho^{\mathrm{ext}}_{s,\alpha}(\mathbf{q}+\mathbf{G}') = \frac{q_\alpha}{q}Z^*_{s,\alpha\beta} + \dots. \tag{43}$$

and the LRC of the dynamical matrix as

$$C^{\mathrm{L}}_{ss',\alpha\beta}(\mathbf{q}) = \frac{4\pi e^2}{V}Z^{\mathrm{c.c.}}_{s,\alpha}(\mathbf{q})\bar{Z}_{s',\beta}(\mathbf{q}) = \frac{4\pi e^2}{V}\epsilon^{-1}(\mathbf{q})\bar{Z}^{\mathrm{c.c.}}_{s,\alpha}(\mathbf{q})\bar{Z}_{s',\beta}(\mathbf{q}) \tag{44}$$

Keeping only the first term of the expansion we get the usual formula for undoped semiconductors

$$C^{\mathrm{L}}_{ss',\alpha\beta}(\mathbf{q}) = \frac{4\pi e^2}{V}\frac{(\sum_\gamma q_\gamma Z^*_{s,\alpha\gamma})(\sum_\gamma q_\gamma Z^*_{s',\beta\gamma})}{\mathbf{q}\cdot\epsilon^\infty\cdot\mathbf{q}}. \tag{45}$$

Notice that this expression is obtained from Eq. (1) of the main text (Eq. 44 of this Supplementary Information) once that one identifies

$$Z_{s,\alpha} = \frac{q^2}{q}\frac{\sum_\gamma q_\gamma Z^*_{s,\alpha\gamma}}{\mathbf{q}\cdot\epsilon^\infty\cdot\mathbf{q}} = \epsilon^{-1}(\mathbf{q})\sum_\gamma \frac{q_\gamma}{q}Z^*_{s,\alpha\gamma} \tag{46}$$

$$\epsilon^{-1}(\mathbf{q}) = \frac{q^2}{\mathbf{q}\cdot\epsilon^\infty\cdot\mathbf{q}} \tag{47}$$

$$\bar{Z}_{s,\beta} = \sum_\gamma \frac{q_\gamma}{q}Z^*_{s',\beta\gamma} \tag{48}$$

The scalar ($\epsilon^{-1}(\mathbf{q})$) and tensorial ($\epsilon^\infty$) form of the response tensor may seem confusing at first, but let's consider the macroscopic Maxwell's equation

$$\nabla\cdot\epsilon^\infty\cdot\nabla\phi^{\mathrm{tot}}(\mathbf{r}) = \rho^{\mathrm{ext}}(\mathbf{r}). \tag{49}$$

Its fourier transform becomes

$$\mathbf{q}\cdot\epsilon^\infty\cdot\mathbf{q}\phi^{\mathrm{tot}}(\mathbf{q}) = 4\pi\rho^{\mathrm{ext}}(\mathbf{q}), \tag{50}$$

$$\phi^{\mathrm{tot}}(\mathbf{q}) = 4\pi\frac{\rho^{\mathrm{ext}}(\mathbf{q})}{\mathbf{q}\cdot\epsilon^\infty\cdot\mathbf{q}} = 4\pi\frac{\epsilon^{-1}(\mathbf{q})}{q^2}\rho^{\mathrm{ext}}(\mathbf{q}) = \Xi^{-1}(\mathbf{q})\rho^{\mathrm{ext}}. \tag{51}$$

In conclusion, the difference between $\epsilon^{-1}(\mathbf{q})$ and $\epsilon^\infty$ is that the first one is the scalar function obtained as the scalar product of the second between wavevectors. Generally speaking, $\epsilon^\infty$ is not the only tensor that enters the determination of $\epsilon^{-1}(\mathbf{q})$, because the expansion may be written as $\epsilon^{-1}(\mathbf{q}) = \frac{q^2}{\mathbf{q}\cdot\epsilon^\infty\cdot\mathbf{q}+\mathbf{q}\mathbf{q}\epsilon^{2,\infty}\mathbf{q}\mathbf{q}} + ...$ where $\epsilon^{2,\infty}$ is now a $3\times3\times3\times3$ tensor [1].

The next higher order term in the expansion for the long range components of the dynamical matrix is

$$C^{\mathrm{L}}_{ss',\alpha\beta}(\mathbf{q}) = \frac{i4\pi e^2}{2V}\frac{(\sum_{\gamma\delta} q_\gamma q_\delta Q_{s,\alpha\gamma\delta})(\sum_\gamma q_\gamma Z^*_{s',\beta\gamma}) - (\sum_\gamma q_\gamma Z^*_{s,\alpha\gamma})(\sum_{\gamma\delta} q_\gamma q_\delta Q_{s',\beta\gamma\delta})}{\mathbf{q}\cdot\epsilon^\infty\cdot\mathbf{q}}, \tag{52}$$

and so on.

**For the case of a doped semiconductor or a metal,** the expansion of Eq. 32 is modified to

$$\frac{\delta\phi_{s',\beta}(\mathbf{q},n,T)}{\hat{\Xi}^{-1}(\mathbf{q},\mathbf{q},n,T)} = \frac{e}{V}G_{s',\beta}(\mathbf{q},n,T). \tag{53}$$

where

$$G_{s',\beta}(\mathbf{q},n,T) = M_{s',\beta}(n,T) - \sum_{\alpha} q_\alpha i Z^*_{s',\beta\alpha}(n,T) - \sum_{\alpha\gamma} \frac{1}{2} q_\alpha q_\gamma Q_{s',\beta\alpha\gamma}(n,T) + \\ + \sum_{\alpha\gamma\delta} i q_\alpha q_\gamma q_\delta \frac{1}{6} O_{s',\beta\alpha\gamma\delta}(n,T) + O(q^4). \tag{54}$$

The nature of the $M_{s',\beta}(n,T)$ term will be elucidated in the following sections. In the meantime, we notice that the above expansion may be recast in the following interesting form

$$G_{s',\beta}(\mathbf{q},n,T) = \sum_{\alpha} q_\alpha F_{s',\alpha\beta}(\mathbf{q}) + \mathcal{C}(\mathbf{q},n,T). \tag{55}$$

The term $\mathcal{C}(\mathbf{q},n,T)$ contains all the effects caused by $n$ and $T$ and it is generated by the intraband contribution to the independent particle polarizability that arise in doped semiconductor and metals. Following the above considerations, at the end we can recast the formula for the unscreened effective charges as

$$\bar{Z}_{s,\alpha}(n,T) = \frac{iV}{eq} \sum_{\mathbf{G}'} \frac{\hat{\Xi}^{-1}(\mathbf{q},\mathbf{q}+\mathbf{G}',n,T)}{\hat{\Xi}^{-1}(\mathbf{q},\mathbf{q},n,T)} \delta\rho^{\rm ext}_{s,\alpha}(\mathbf{q}+\mathbf{G}') = \frac{i}{q} M_{s,\alpha}(n,T) + \frac{q_\alpha}{q} Z^*_{s,\alpha\beta}(n,T) + \dots . \tag{56}$$

and the LRC of the dynamical matrix as

$$C^{\rm L}_{ss',\alpha\beta}(\mathbf{q}) = \frac{4\pi e^2}{V} Z^{\rm c.c.}_{s,\alpha}(\mathbf{q},n,T) \bar{Z}_{s',\beta}(\mathbf{q},n,T) = \frac{4\pi e^2}{V} \epsilon^{-1}(\mathbf{q},n,T) \bar{Z}^{\rm c.c.}_{s,\alpha}(\mathbf{q},n,T) \bar{Z}_{s',\beta}(\mathbf{q},n,T) \tag{57}$$

We remind that the conclusions of the main text imply that $\bar{Z}_{s,\alpha}(\mathbf{q},n,T)$, that depends only on the wings of the dielectric matrix, is less sensitive to doping than the head $\epsilon^{-1}(\mathbf{q},n,T)$. Qualitatively, this can be explained within a Thomas-Fermi approach, where $\epsilon(\mathbf{q}) \approx \epsilon^\infty + k^2_{\rm TF}(T)/q^2$. One can then replace $q^2/\left(\mathbf{q}\cdot\overleftrightarrow{\epsilon}^\infty\cdot\mathbf{q}\right) \to q^2/\left(k^2_{\rm TF}(T) + \mathbf{q}\cdot\overleftrightarrow{\epsilon}^\infty\cdot\mathbf{q}\right)$ in the formula for the LRCs, thus expressing them in a manifestly analytic form for each level of doping (even vanishing).

### LRC of the EPI

The EPI can be expressed as [6]

$$\langle \psi_{m\mathbf{k}+\mathbf{q}} | g_{\mathbf{q},\nu}(\mathbf{r}) | \psi_{n\mathbf{k}} \rangle = \sum_{\mathbf{G}\mathbf{G}'\mathbf{G}''} u^{\rm c.c}_{m,\mathbf{k}+\mathbf{q}}(\mathbf{G}) u_{n,\mathbf{k}}(\mathbf{G}') \epsilon^{-1}(\mathbf{q}+\mathbf{G}'-\mathbf{G},\mathbf{q}+\mathbf{G}'') g^{\mathbf{q},\rm b}_\nu(\mathbf{G}''), \tag{58}$$

where

$$g_{\nu}^{\mathbf{q},\mathrm{b}}(\mathbf{G}'') = i\frac{4\pi e^2}{V}\sum_{s,\alpha}\frac{Z_s}{|\mathbf{q}+\mathbf{G}''|^2}(q_\alpha + G''_\alpha)e^{-i\mathbf{G}''\cdot\boldsymbol{\tau}_s}e^{\nu}_{s,\alpha}(\mathbf{q})l^{\nu}_{\mathbf{q}}\left(\frac{M_0}{M_s}\right)^{1/2}, \tag{59}$$

and

$$l^{\nu}_{\mathbf{q}} = [\frac{\hbar}{2M_0\omega_{\mathbf{q},\nu}}]^{1/2}. \tag{60}$$

is the phonon zero-point motion amplitude, where $M_0$ is an arbitrary reference mass. As for the dynamical matrix, we express the above quantities as a function of the $\Xi^{-1}$ matrix and recognize the long range part as

$$g^{\mathrm{L}}_{\nu,mn}(\mathbf{k},\mathbf{q}) = i\frac{4\pi e^2}{V}\sum_{\mathbf{G}\mathbf{G}'\mathbf{G}''}\sum_{s,\alpha}u^{\mathrm{c.c}}_{m\mathbf{k}+\mathbf{q}}(\mathbf{G})u_{n\mathbf{k}}(\mathbf{G}')\times$$
$$\times\frac{\hat{\Xi}^{-1}(\mathbf{q},\mathbf{q}+\mathbf{G}'')\hat{\Xi}^{-1,\mathrm{c.c.}}(\mathbf{q},\mathbf{q}+\mathbf{G}'-\mathbf{G})}{\hat{\Xi}^{-1}(\mathbf{q},\mathbf{q})}Z_s(q_\alpha+G''_\alpha)e^{-i\mathbf{G}''\cdot\boldsymbol{\tau}_s}e^{\nu}_{s,\alpha}(\mathbf{q})l^{\nu}_{\mathbf{q}}\left(\frac{M_0}{M_s}\right)^{1/2}, \tag{61}$$

from which follows

$$g^{\mathrm{L}}_{\nu,mn}(\mathbf{k},\mathbf{q}) = -\frac{4\pi e^2}{V}\sum_{\mathbf{G}\mathbf{G}'}\sum_{s,\alpha}u^{\mathrm{c.c}}_{m,\mathbf{k}+\mathbf{q}}(\mathbf{G})u_{n,\mathbf{k}}(\mathbf{G}')\times$$
$$\times\hat{\Xi}^{-1,\mathrm{c.c.}}(\mathbf{q},\mathbf{q}+\mathbf{G}'-\mathbf{G})\bar{Z}_{s,\alpha}(\mathbf{q})e^{\nu}_{s,\alpha}(\mathbf{q})l^{\nu}_{\mathbf{q}}\left(\frac{M_0}{M_s}\right)^{1/2} \tag{62}$$

**For an undoped semiconductor**, inserting the expression for the effective charges we obtain

$$g^{\mathrm{L}}_{\nu,mn}(\mathbf{k},\mathbf{q}) = -\frac{4\pi e^2}{V}\sum_{\mathbf{G}\mathbf{G}'}\sum_{s,\alpha}u^{\mathrm{c.c}}_{m,\mathbf{k}+\mathbf{q}}(\mathbf{G})u_{n,\mathbf{k}}(\mathbf{G}')\times$$
$$\times\hat{\Xi}^{-1,\mathrm{c.c.}}(\mathbf{q},\mathbf{q}+\mathbf{G}'-\mathbf{G})\sum_{\beta}q_\beta F_{s,\alpha\beta}(\mathbf{q})e^{\nu}_{s,\alpha}(\mathbf{q})l^{\nu}_{\mathbf{q}}\left(\frac{M_0}{M_s}\right)^{1/2} \tag{63}$$

The leading long range order of the above expression becomes

$$g^{\mathrm{L}}_{\nu,mn}(\mathbf{k},\mathbf{q}) = i\frac{4\pi e^2}{V}\sum_{\mathbf{G}}\sum_{s}u^{\mathrm{c.c}}_{m\mathbf{k}+\mathbf{q}}(\mathbf{G})u_{n\mathbf{k}}(\mathbf{G})\frac{\sum_{\alpha\beta}q_\beta Z^*_{s,\alpha\beta}e^{\nu}_{s,\alpha}(\mathbf{q})}{\mathbf{q}\cdot\epsilon^{\infty}\cdot\mathbf{q}}l^{\nu}_{\mathbf{q}}\left(\frac{M_0}{M_s}\right)^{1/2}. \tag{64}$$

The next higher order terms are:

$$g^{\mathrm{L}}_{\nu,mn}(\mathbf{k},\mathbf{q}) = \frac{1}{2}\frac{4\pi e^2}{V}\sum_{\mathbf{G}}\sum_{s}u^{\mathrm{c.c}}_{m\mathbf{k}+\mathbf{q}}(\mathbf{G})u_{n\mathbf{k}}(\mathbf{G})\frac{\sum_{\alpha\beta\gamma}q_\beta q_\gamma Q_{s,\alpha\beta\gamma}e^{\nu}_{s,\alpha}(\mathbf{q})}{\mathbf{q}\cdot\epsilon^{\infty}\cdot\mathbf{q}}l^{\nu}_{\mathbf{q}}\left(\frac{M_0}{M_s}\right)^{1/2}+$$
$$i\frac{4\pi e^2}{V}\sum_{\mathbf{G}\neq\mathbf{G}'}\sum_{s}u^{\mathrm{c.c}}_{m\mathbf{k}+\mathbf{q}}(\mathbf{G})u_{n\mathbf{k}}(\mathbf{G}')\left[-\mathbf{q}\cdot\mathbf{A}'^{\mathrm{c.c}}(\mathbf{G}'-\mathbf{G})\right]\frac{\sum_{\alpha\beta}q_\beta Z^*_{s,\alpha\beta}e^{\nu}_{s,\alpha}(\mathbf{q})}{\mathbf{q}\cdot\epsilon^{\infty}\cdot\mathbf{q}}l^{\nu}_{\mathbf{q}}\left(\frac{M_0}{M_s}\right)^{1/2}. \tag{65}$$

The second term of the above expression can be recast in terms of the potentials appearing in the DFT Hamiltonian, as explained in Ref. [5]. Such term is expected to be smaller than the term dependent on the quadrupole tensor [7]; also, it is non null only for the optical coupling, where the Fröhlich coupling is expected to be far more important for polar materials, so that it is usually neglected with a small error.

**For a doped semiconductor or a metal**, as explained in detail for the case of the dynamical matrix, Eq. 62 still holds in presence of finite doping and temperature, expliciting the dependence $\hat{\Xi}^{-1,\text{c.c.}}(\mathbf{q}, \mathbf{q} + \mathbf{G}' - \mathbf{G}) \rightarrow \hat{\Xi}^{-1,\text{c.c.}}(\mathbf{q}, \mathbf{q} + \mathbf{G}' - \mathbf{G}, n, T)$ and $Z_{s,\alpha}(\mathbf{q}) \rightarrow Z_{s,\alpha}(\mathbf{q}, n, T)$. In this case, our extension of the expressions of the LRCs to include $Z_{s,\alpha}$ instead of $Z^*_{s,\alpha\beta}$ is of fundamental importance, as we will see later. To conclude the theoretical section, we represent the theoretical steps that bring to the derivation of the LRCs of the dynamical matrix and of of the EPI in Fig. 1.

## DETAILED COMPUTATIONAL INFORMATION

To perform the first-principles calculations we use a private version of the QUANTUM ESPRESSO code [8], adapted in order to extract the total macroscopic charge density change on each atom from DFPT and to compute the dielectric screening. We use PBE-GGA functionals [9] and norm-conserving pseudopotentials that are the same as used in Ref. [10] and are available at `10.24435/materialscloud:b2-j5`. The lattice parameter used is $a = 5.3596$Ang. The energy cutoff for the plane wave basis set is 80Ry.

We sample the BZ with telescopic grids centered around $\Gamma$, that are built starting from the reciprocal space in crystallographic coordinates (in units of $2\pi/a$) with a generalization of the procedure developed in Ref. [11]. In such coordinates, the first BZ is a cube that, within the usual Monkhorst-Pack scheme, would be subdivided in $N \times N \times N$ equivalent smaller cubes. Instead, our procedure is iterative and acts on a given cube $\mathcal{C}$ generated at the $n$-th iteration by subdividing it in 27 equivalent cubes if a certain request is satisfied. To describe the request, we first define a mimimum and a maximum depth for the level of the telescopic grids ($m$ and $M$). If $n < m$ then $\mathcal{C}$ is always subdivided in 27 equal sub-cubes whose centers are added to the list of points of the grid. When $n >= m$, if the Cartesian coordinates (in units of $2\pi/a$) of the center of $\mathcal{C}$, $\mathbf{r}_\mathcal{C}$, satisfies the request

$$|\mathbf{r}_\mathcal{C}| < \frac{1}{N} 4^{\frac{M-n}{l}} \tag{66}$$

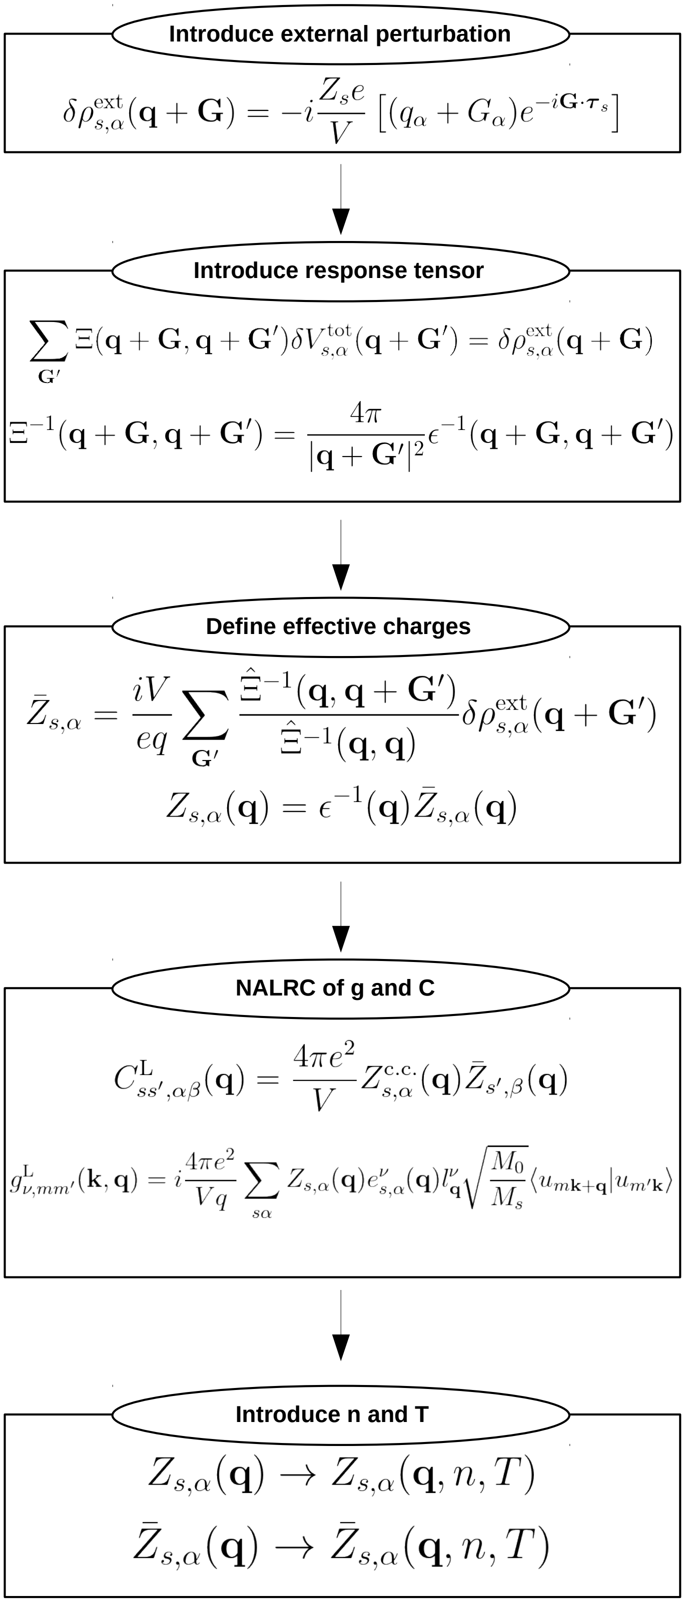


FIG. 1: Workflow of the theoretical steps that bring to Eq. (1) and (2) of the main text.

where $N$ and $l$ are conveniently chosen parameter, then $\mathcal{C}$ is subdivided in 27 equal sub-cubes whose centers are added to the list of points of the grid, otherwise we stop the procedure for $\mathcal{C}$ and move to the next cube. The weights for a point generated at the $n$-th iteration of the algorithm is $w_i = 27^{-n}$. The points and weights are then reduced using the point group symmetry operations of the crystal. The grid used in this work for the doped case is generated with $M = 6$, $m = 4$, $N = 15$ and $l = 2$, corresponding to a grid containing 16325 points in the Irreducible Wedge (IW) of the BZ, while for the undoped case we use a grid generated with $M = 6$, $m = 4$, $N = 30$ and $l = 2$ containing 12494 points in the IW. Only in the neutral case, the charge density changes are very similar to the ones obtained employing uniform grids, because in this case the description of the various quantities is not sensitive to the neighborhoods of the $\Gamma$ point. An example of telescopic grid generated with $M = 6$, $m = 2$, $N = 30$ and $l = 2$ is shown in Fig. 2. In our calculations we use grids that in the densest region are equivalent to Monkhorst-Pack grids of dimension $729^3$.

The Wannier interpolation is performed using a private version of EPW [12], adapted in order to treat the LRC of the interactions as described in the main text of the article. The maximally localized Wannier functions (MLWF) are obtained on electronic meshes of $16^3$, starting from $sp^3$ atomic orbital projections, with the same input used in Ref. [10]. The grid for the Fourier interpolation of the phonons is of dimensions $8^3$.

The nulling of the macroscopic component of the electrostatic potential is achieved by putting to zero the change of the local part of the pseudopotential and of the Hartree and exchange-correlation potentials at $\mathbf{G} = 0$ (where $\mathbf{G}$ is a generic reciprocal lattice vector) during the self-consistent solution of the Sternheimer equation in presence of the external perturbation connected to $v_{s,\alpha}(\mathbf{q})$ (more details are given in the following sections); this procedure has been implemented in our private version of the QUANTUM ESPRESSO code.

As mentioned in the main text, the calculation of the first-principles dielectric function is obtained following the method of Ref. [13] implemented in a private version of the QUANTUM ESPRESSO code, at a computational cost which is roughly the equivalent of a phonon calculation at the point $\mathbf{q}$ divided by the total number of phonon modes.

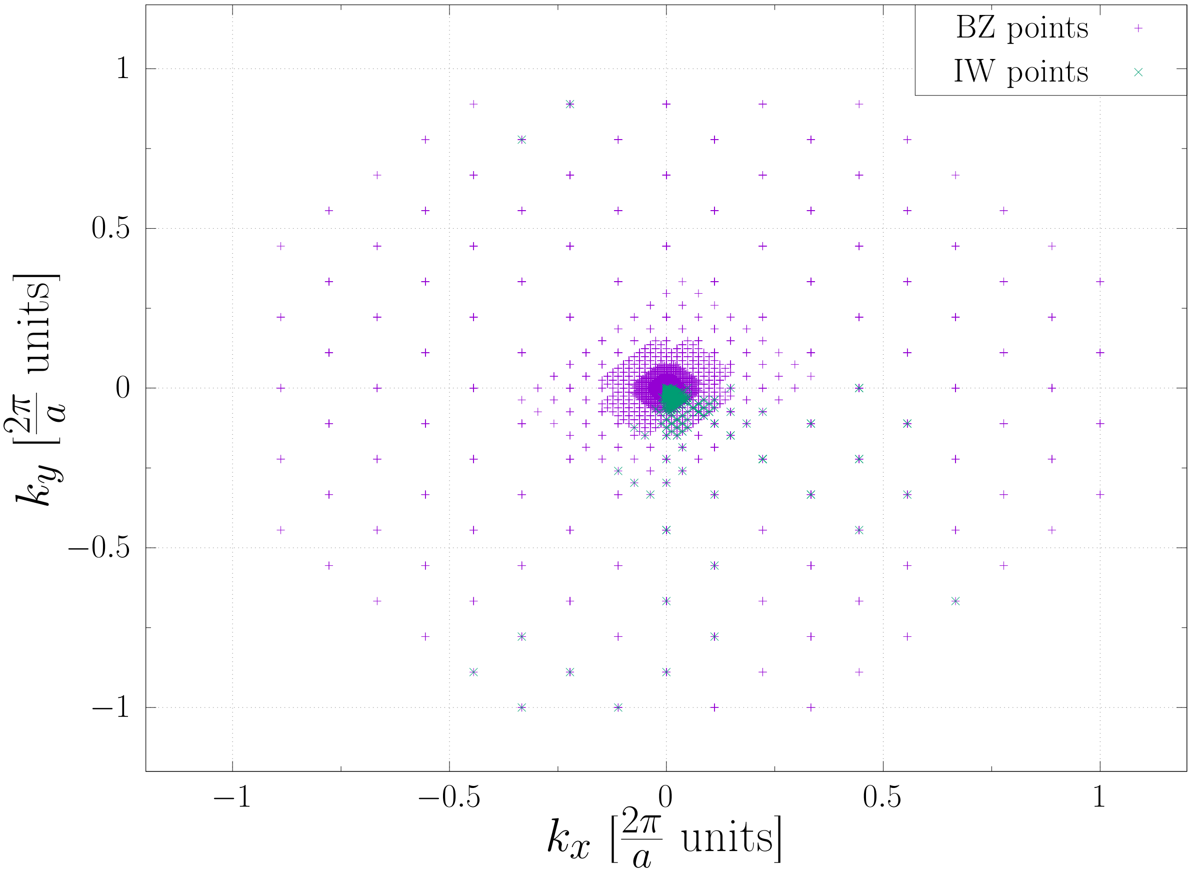


FIG. 2: *Example of telescopic grid with unreduced BZ points (violet crosses) and symmetry reduced IW points (green crosses).*

**Rules for the charge determination along cartesian directions**

We consider the rules for the cubic case of 3C-SiC (group $F\bar{4}3m$). The direct lattice vectors are defined as:

$$\mathbf{v}_1 = a\left(-\frac{1}{2}, 0, \frac{1}{2}\right), \tag{67}$$

$$\mathbf{v}_2 = a\left(0, \frac{1}{2}, \frac{1}{2}\right), \tag{68}$$

$$\mathbf{v}_3 = a\left(-\frac{1}{2}, \frac{1}{2}, 0\right). \tag{69}$$

Since the effective charge tensors are local, atomic-dependent quantities, one may exploit the site-symmetry and the point-group properties of associated Wyckoff positions to determine

the symmetry-allowed non-zero components of the tensors. Specifically, for a generic tensor $O$ it must hold that $U_k^\dagger O_k U_k = O_k$, where $k$ is the atomic index and $U_k$ represents a symmetry operation belonging to the site-symmetry point-group of atom $k$. Si and C atoms share the same $T_d$ site-symmetry in 3C-SiC, and the allowed components for polar tensors fulfill the following relationships:

$$Z_{s,\alpha\beta} = (-1)^s Z \delta_{\alpha\beta} \tag{70}$$

$$Q_{s,\alpha\beta\gamma} = Q_s |\epsilon_{\alpha\beta\gamma}| \tag{71}$$

$$O_{s,\alpha\beta\gamma\delta} = \begin{cases} O_s^1 & \alpha = \beta = \gamma = \delta \\ O_s^2 & (\alpha = \beta) \neq (\gamma = \delta) \\ O_s^3 & (\alpha = \gamma) \neq (\beta = \delta) \end{cases}, \tag{72}$$

where $\epsilon_{\alpha\beta\gamma}$ is the Levi-Civita tensor. In particular, the change of sign for $Z_{s,\alpha\beta}$ is a consequence of a sum rule which may be derived following Ref. [4], and that corresponds to the effective charge neutrality condition. The non-zero components of the cartesian tensors that do not depend on the atom index—such as $\epsilon^\infty$—are instead determined by the crystallographic point group $G$, imposing that $U^\dagger O U = O \quad \forall U \in G$ . It follows for the $F\bar{4}3m$ group that

$$\epsilon^\infty_{\alpha\beta} = \epsilon^\infty \delta_{\alpha\beta}. \tag{73}$$

Similarly, at the leading order in the $\mathbf{q}$ expansion we have that

$$\epsilon^{-1}(\mathbf{q}) = \frac{\mathbf{q}}{q} \cdot \tilde{\epsilon}^{-1}(|\mathbf{q}|) \cdot \frac{\mathbf{q}}{q} \tag{74}$$

where

$$\tilde{\epsilon}^{-1}(|\mathbf{q}|)_{\alpha\beta} = \tilde{\epsilon}^{-1}(|\mathbf{q}|)\delta_{\alpha\beta}. \tag{75}$$

The same arguments above can be repeated for each symmetry group of any material. In table I we give the explicit expressions of the Taylor expansion Eq. (4) in the main text specialized to high-symmetry lines, enforcing the symmetry properties of effective charge tensors.

## DYNAMICAL QUADRUPOLES

As described in the main text of this article and in the previous sections, we can in principle determine the effective charge tensors at an arbitrary order induced by an external

| $\delta\rho$ | Cartesian direction | | |
|---|---|---|---|
| | $[q,0,0]$ | $[0,q,0]$ | $[0,0,q]$ |
| $\delta\rho_{s,x}$ | $q^2\frac{-i(-1)^sZq+i/6O_s^1q^3+O(q^4)}{\mathbf{q}\cdot\epsilon^\infty\cdot\mathbf{q}+\mathbf{qq}\cdot\epsilon^4\cdot\mathbf{qq}+O(q^6)}$ | 0 | 0 |
| $\delta\rho_{s,y}$ | 0 | $q^2\frac{-i(-1)^sZq+i/6O_s^1q^3+O(q^4)}{\mathbf{q}\cdot\epsilon^\infty\cdot\mathbf{q}+\mathbf{qq}\cdot\epsilon^4\cdot\mathbf{qq}+O(q^6)}$ | 0 |
| $\delta\rho_{s,z}$ | 0 | 0 | $q^2\frac{-i(-1)^sZq+i/6O_s^1q^3+O(q^4)}{\mathbf{q}\cdot\epsilon^\infty\cdot\mathbf{q}+\mathbf{qq}\cdot\epsilon^4\cdot\mathbf{qq}+O(q^6)}$ |

| $\delta\rho$ | Cartesian direction | |
|---|---|---|
| | $[0,q/\sqrt{2},q/\sqrt{2}]$ | $[q/\sqrt{3},q/\sqrt{3},q/\sqrt{3}]$ |
| $\delta\rho_{s,x}$ | $q^2\frac{-Q_sq^2/2+O(q^4)}{\mathbf{q}\cdot\epsilon^\infty\cdot\mathbf{q}+\mathbf{qq}\cdot\epsilon^4\cdot\mathbf{qq}+O(q^6)}$ | $q^2\frac{-i(-1)^sZq/3^{1/2}-Q_sq^2/3+i/6(O_s^1+2O_s^2+2O_s^3)q^3/3^{3/2}+O(q^4)}{\mathbf{q}\cdot\epsilon^\infty\cdot\mathbf{q}+\mathbf{qq}\cdot\epsilon^4\cdot\mathbf{qq}+O(q^6)}$ |
| $\delta\rho_{s,y}$ | $q^2\frac{-i(-1)^sZq/2^{1/2}+i/6(O_s^1+O_s^2+O_s^3)q^3/2^{3/2}+O(q^4)}{\mathbf{q}\cdot\epsilon^\infty\cdot\mathbf{q}+\mathbf{qq}\cdot\epsilon^4\cdot\mathbf{qq}+O(q^6)}$ | $q^2\frac{-i(-1)^sZq/3^{1/2}-Q_sq^2/3+i/6(O_s^1+2O_s^2+2O_s^3)q^3/3^{3/2}+O(q^4)}{\mathbf{q}\cdot\epsilon^\infty\cdot\mathbf{q}+\mathbf{qq}\cdot\epsilon^4\cdot\mathbf{qq}+O(q^6)}$ |
| $\delta\rho_{s,z}$ | $q^2\frac{-i(-1)^sZq/2^{1/2}+i/6(O_s^1+O_s^2+O_s^3)q^3/2^{3/2}+O(q^4)}{\mathbf{q}\cdot\epsilon^\infty\cdot\mathbf{q}+\mathbf{qq}\cdot\epsilon^4\cdot\mathbf{qq}+O(q^6)}$ | $q^2\frac{-i(-1)^sZq/3^{1/2}-Q_sq^2/3+i/6(O_s^1+2O_s^2+2O_s^3)q^3/3^{3/2}+O(q^4)}{\mathbf{q}\cdot\epsilon^\infty\cdot\mathbf{q}+\mathbf{qq}\cdot\epsilon^4\cdot\mathbf{qq}+O(q^6)}$ |

TABLE I: *Taylor expansion of the total charge induced by a collective displacement of wavevector* $\mathbf{q}$ *of the atom* $s$*, along different special lines. The expressions are given for a reciprocal space vector of length* $q$*.*

atomic perturbation $\delta\rho^{\text{ext}}_{s,\alpha}(\mathbf{q}+\mathbf{G})$. In the main text we showed that the Born effective charges perfectly describe the leading asymptotic order of the real part of the effective charges computed via ab-initio calculations for the undoped setup; even in presence of doping their unaltered value can be used inside the expression for $Z_{s,\alpha}$ to reproduce *ab-initio* calculations. The computation of the second order expansion of $\bar{Z}_{s,\alpha}(\mathbf{q})$, related to the dynamical effective quadrupole tensor, can be performed looking at the imaginary part of $\bar{Z}_{s,\alpha}(\mathbf{q})$ (for an alternative DFPT approach see Ref. [14]). It is in this case found that $\text{Im}\bar{Z}_{s,z}(\mathbf{q},n,T)$ is affected by doping, while its sum over the atoms (proportional to the unscreened frozen ion (FI) piezoelectric tensor [15] $\bar{e}^{\text{FI}}_{\alpha\beta\gamma}\propto Q_{Si,\alpha\beta\gamma}+Q_{C,\alpha\beta\gamma}$) is much less influenced. Interestingly, for atoms with only one atomic species in the long wavelength limit the LRC of the interaction between electron and acoustic phonons depends only on $e^{\text{FI}}$. We will show this now.

We first show in Fig. 3 the opposite of the imaginary part of the effective charges divided by $q/2$—which is the quadrupole tensor divided by $\epsilon^\infty$—computed via ab-initio in

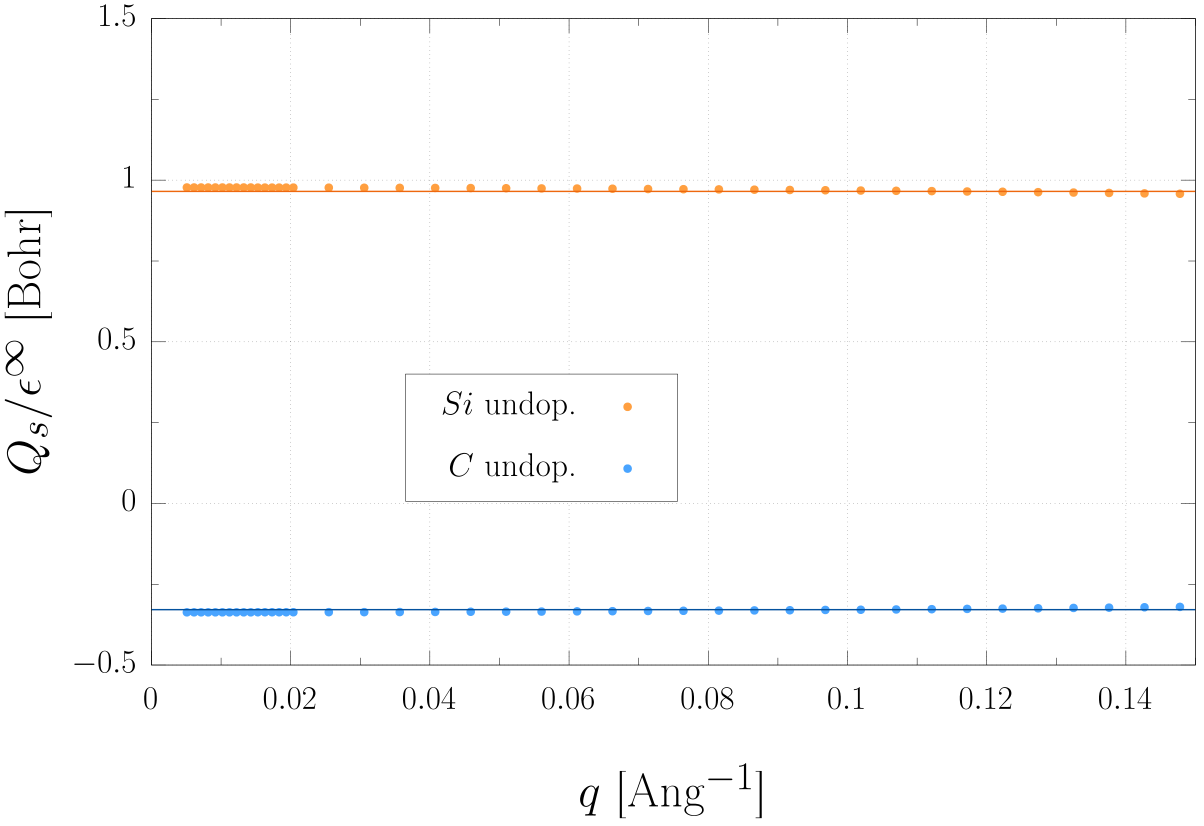


FIG. 3: *Fitting of quadrupole moments for the undoped case as a function of $q$ along the line $\mathbf{q} = \left(q/\sqrt{2}, q/\sqrt{2}, 0\right)$.*

the undoped setup, along a specific line in reciprocal space; knowing $\epsilon^\infty$ from first principles calculations, we can extract the values of the quadrupole tensors which we find to be $Q_{Si} = 6.6783$ and $Q_C = -2.2733$. We sum up the material dependent quantities for the undoped setup in Tab. II.

| Atom | $Z_{xx}$ | $Q_{xyz}$ [Bohr] | $\epsilon^\infty$ |
|---|---|---|---|
| Si | 2.699 | 6.6783 | 6.9179 |
| C | -2.699 | -2.2733 | 6.9179 |

TABLE II: *Sum up of material dependent quantities.*

In Fig. 4b and 4a instead we show directly, for matter of convenience, the real part of

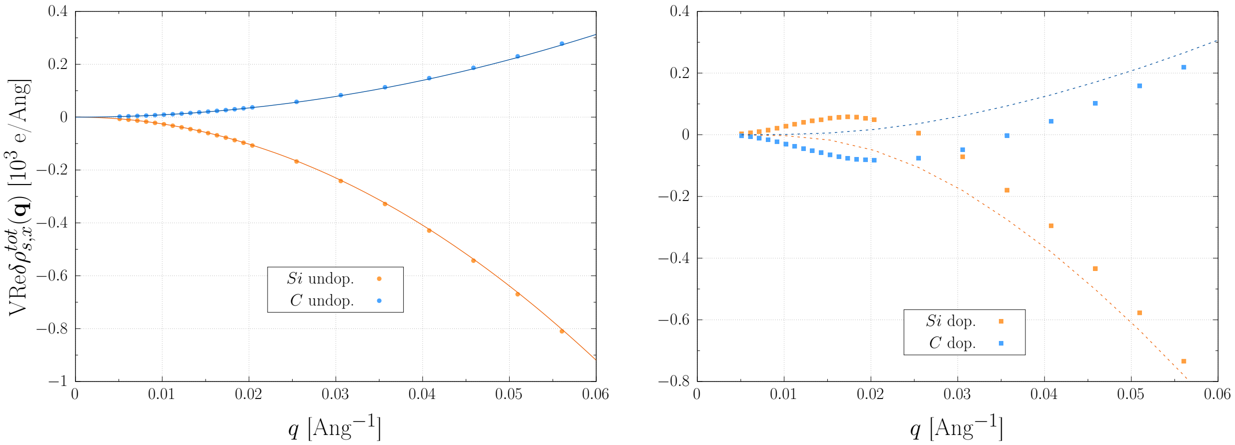


(a) (b)

FIG. 4: *Imaginary part of the total charge density change as a function of $q$ along the line $\mathbf{q} = \left(q/\sqrt{2}, q/\sqrt{2}, 0\right)$, for both the atoms in 3C-SiC in the a) undoped case and b) doped case with a carrier concentration of $n = 4.827 \times 10^{15}\, cm^{-3}$. The continuous lines are drawn using the asymptotic expressions for the charge density change in the undoped case, while the dashed ones are for the doped case.*

the charge density change in the undoped and doped cases (which is proportional to the imaginary part of the effective charge multiplied by $q$, following Eq. 3). In the doped case, we can see that at small $\mathbf{q}$ variations with respect to the expected behaviour—obtained screening the values of $Q_{Si}$ and $Q_C$ with the RPA approximation to the inverse dielectric function—are introduced on both atoms. These variations are equal in value on both atoms (but with opposite signs) and are due to the effect of doping on the wings of the dielectric matrix. To understand this better, we plot the real part of the *unscreened* total charge density $\delta\bar{\rho}^{\mathrm{tot}}_{s,\alpha}(\mathbf{q})$ in Fig. 5a. We here notice that departures from the expected behaviour that arise in the charge density change cannot be easily described by the expansion given in Eq. 54. In this case it is better to consider Eq. 55: we can say that $\mathcal{C}_{s,\alpha}(\mathbf{q}, n, T)$ is different from zero in the region where the dielectric response acquires metallic features, with the property that the sum over the atoms is zero: $\sum_s \lim_{\mathbf{q}\to 0} \mathcal{C}_{s,\alpha}(\mathbf{q}, n, T) = 0$—notice that in general (but not for 3C-SiC) $\lim_{\mathbf{q}\to 0} \mathcal{C}_{s,\alpha}(\mathbf{q}, n, T) \neq 0$ as discussed later. From Fig. 5a we notice that $\mathcal{C}_{s,\alpha}(\mathbf{q}, n, T)$ is substantially different from zero for $\frac{q}{\sqrt{2}} < 0.03$, which is the region where screening departs from the semiconductor behaviour (see main text), while it vanishes

for larger wavevectors. As anticipated, $\mathcal{C}_{s,\alpha}(\mathbf{q}, n, T)$ is therefore due to metallization, i.e. to the change of the intraband term and the appearence of a contribution of an intraband term to $\chi^0$ which in turn determines the induced charge density.

Accordingly with what commented above, if we plot the sum of the effective charges over the atoms (Fig. 5b), which is proportional to the screened frozen-ion piezoelectric tensor $e^{\rm FI}_{\alpha\beta\gamma} = \epsilon^{-1}(\mathbf{q},\mathbf{q})\bar{e}^{\rm FI}_{\alpha\beta\gamma} \propto \epsilon^{-1}(\mathbf{q},\mathbf{q})\,(Q_{Si,\alpha\beta\gamma} + Q_{C,\alpha\beta\gamma})$, we find that $\bar{e}^{\rm FI}_{\alpha\beta\gamma}(n) \approx \bar{e}^{\rm FI}_{\alpha\beta\gamma}(n=0)$ so that all the doping dependence of the piezoelectric tensor is implicit in the dielectric screening. This is an interesting observation since, for atoms with only one atomic species in the long wavelength limit the LRC of the interaction between electron and acoustic phonons depends only on $e^{\rm FI}$.

## FERMI ENERGY SHIFT

We now discuss in which cases $\lim_{\mathbf{q}\to 0} \mathcal{C}_{s,\alpha}(\mathbf{q}, n, T) = M_{s,\alpha}(n, T)$ is different from zero. We recall that the term $M_{s,\alpha}$ is present only in doped semiconductors or metals. We start from some general considerations regarding the solution of the linear response problem.

The condition of zero macroscopic field $\delta V^{\rm tot}_{s,\alpha}(\mathbf{q}) = 0$ is imposed by putting to zero the macroscopic change of the local part of the pseudopotential and of the Hartree potential. This condition is automatically imposed by the QUANTUM EPSRESSO code at $\mathbf{q} = 0$, so that the QE code at $\mathbf{q} = 0$ is solving the linear response problem by computing the unscreened charge density change.

We know that the screened charge density change has to go to zero for $\mathbf{q} \to 0$ for the condition of charge neutrality; the unscreened charge density change instead is not always constrained to go to zero for $\mathbf{q} \to 0$. In semiconductors, since $\epsilon^{-1} \to 1/\epsilon^{\infty}$, the analytic expansion of $\delta\bar{\rho}_{s,\alpha}(\mathbf{q})$ has to be at least linear in $\mathbf{q}$, so that $\delta\rho_{s,\alpha}(\mathbf{0}) = 0$ (microscopically, this follows from the fact that the wing of the indipendent particle polarizability is at least linear in $\mathbf{q}$ so that Eq. 35 is in turn at least linear in $\mathbf{q}$); for metals, since in three dimensions the metallic screening for small wavevectors scales as $q^{-2}$, $\delta\bar{\rho}_{s,\alpha}(\mathbf{0})$ can also evaluate to a certain constant $M_{s,\alpha}$. In this case, if one performs the calculation at $\mathbf{q} = 0$ imposing that the change of the Hartree potential and of the long range part of the local pseudopotential and imposing the charge neutrality condition (as done in QE), i.e. imposing $\delta\bar{\rho}_{s,\alpha}(\mathbf{0}) = 0$ applying the so-called 'Fermi energy shift' (FES) [2] i.e. adding $-M_{s,\alpha}$ to the density at

$\mathbf{q} = 0$, one obtains a discontinuous behaviour of the unscreened charge density change between $\mathbf{q} = 0$ and its neighborhood—it can be verified numerically that removing the FES the continuity of the unscreened charge change is obtained. This discontinuity is obtained every time in a system $M_{s,\alpha}$ is non constrained to be zero for symmetry reasons; if $M_{s,\alpha}$ instead is costrained to be zero the continuity of the unscreened charge density change is assured, since $\delta\bar{\rho}_{s,\alpha}(\mathbf{0}) = 0$ by the intrinsic properties of the system. The condition to have a zero $M_{s,\alpha}$, or equivalently $\delta\bar{\rho}_{s,\alpha}(\mathbf{0}) = 0$, is the same required for having zero forces by symmetry on all atoms of the system; the analogy with the forces also implies that the sum over the atoms of the constant term goes to zero at $\mathbf{q} = 0$.

We now translate the above conclusions in terms of change of the total potential $\delta V^{\text{tot}}_{s,\alpha}(\mathbf{q})$, using the equation $\hat{\Xi}^{-1}(\mathbf{q},\mathbf{q})\delta\bar{\rho}^{\text{tot}}_{s,\alpha}(\mathbf{q}) = 4\pi\epsilon^{-1}(\mathbf{q},\mathbf{q})/q^2\delta\bar{\rho}^{\text{tot}}_{s,\alpha}(\mathbf{q}) = \delta V^{\text{tot}}_{s,\alpha}(\mathbf{q})$ derived in the above sections. If the system symmetries allows for a non-zero $M_{s,\alpha}$, and using an asymptotic form for $\epsilon^{-1}(\mathbf{q}) = \frac{q^2}{4\pi e^2 n(E_F)}$, we obtain $\lim_{\mathbf{q}\to 0}\delta V^{\text{tot}}_{s,\alpha}(\mathbf{q}) = \frac{1}{eV}\frac{M_{s,\alpha}}{n(E_F)}$, while at $\mathbf{q} = 0$ the condition under which the linear response problem is solved is $\delta V^{\text{tot}}_{s,\alpha}(\mathbf{0}) = 0$. This has an impact on the evaluation of the LRC of the EPCI (which is no more non-analytic for metals but still has the formal expression as given in the main text), since its espression as a function of the change of total potential is, from Eq. 63,

$$g^{\text{L}}_{\nu,mn}(\mathbf{k},\mathbf{q}) = -4\pi e \sum_{\mathbf{G}\mathbf{G}'}\sum_{s,\alpha} u^{\text{c.c}}_{m,\mathbf{k}+\mathbf{q}}(\mathbf{G})u_{n,\mathbf{k}}(\mathbf{G}')\times$$
$$\times\hat{\Xi}^{-1,*}(\mathbf{q},\mathbf{q}+\mathbf{G}'-\mathbf{G})\frac{\delta V^{\text{tot}}_{s,\alpha}(\mathbf{q})}{\Xi^{-1}(\mathbf{q},\mathbf{q})}e^{\nu}_{s,\alpha}(\mathbf{q})l^{\nu}_{\mathbf{q}}\left(\frac{M_0}{M_s}\right)^{1/2}. \tag{76}$$

It is then clear that if a non-zero $M_{s,\alpha}$ is allowed by symmetry the LRC of the EPCI is discontinuous, because the LRC is put to zero by QE at $\mathbf{q} = \mathbf{0}$ but not in its neighborhood; it has therefore to be made continuous by adding to the change of the total potential in $\mathbf{q} = 0$ the value $-\frac{1}{eV}\frac{M_{s,\alpha}}{n(E_F)}$; the continuity is needed to ensure that the Wannier interpolation works well (even without treating explicitly the LRC since everything is analytic). The impact on the frequencies of a non-zero $M_{s,\alpha}$ is instead not seen since there is a further power of $q$ at the numerator lead to the continuity of the dynamical matrix.

The above derivation was thought thinking about a metal; for a doped semiconductor the conclusions are the same if one consider the part of the density response $\mathcal{M}_{s,\alpha}(\mathbf{q})$ which is due to the intraband contribution to the independent particle polarizability, with the caveat that the term dependent on $n(E_F)$ is to be changed with the correct coefficients of

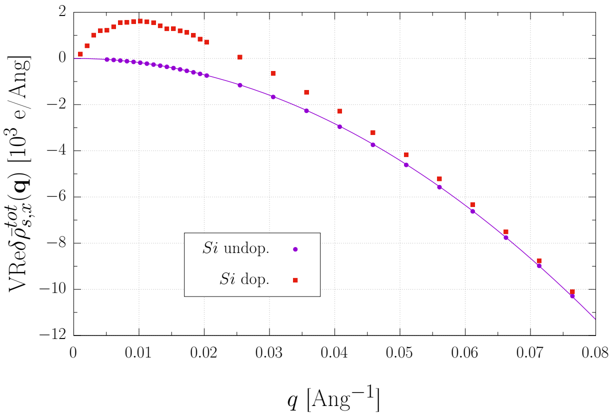


(a)

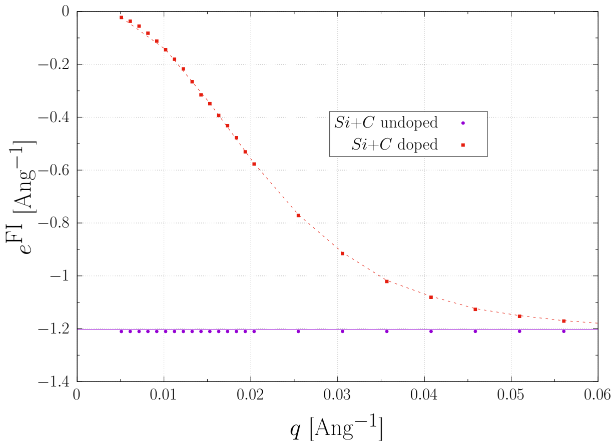


(b)

FIG. 5: *a) Real part of the unscreened total charge density $\delta\bar{\rho}^{tot}_{s,x}(\mathbf{q})$ as a function of $q$ along the line $\mathbf{q} = \big(q/\sqrt{2}, q/\sqrt{2}, 0\big)$, in the undoped and doped setups. b) Screened frozen ion piezoelectric tensor—proportional to the sum of the screened dynamical effective quadrupoles—along the same line, in the undoped and doped setups. The continuous lines are drawn screening the $\bar{e}^{FI}$ computed in the undoped setup with $\epsilon^{\infty}$, while the dashed ones are drawn screenening it with $\epsilon^{-1}(\mathbf{q}, n, T)$.*

$\epsilon^{-1}$ as a function of $q^2$. In our approach, this problem is automatically cured by computing and interpolating the SRC of the undoped model (therefore wihtouth FES) and adding the correct form of the LRC, defining the value of the EPCI at $\mathbf{q} = 0$ as the sum of the SRC at $\mathbf{q} = 0$ plus the limiting value of the LRC.

## VALIDITY OF THE APPROXIMATIONS TO DIELECTRIC SCREENING OF THE MAIN TEXT

In this section we analyse the impact that the various approximations to dielectric screening of the main text have on the description of the $\epsilon^{-1}(\mathbf{q})$ response function. We start from an expression for the independent particle polarizability of the form

$$\chi^0(\mathbf{q}, n, T) \approx \chi^{0,\mathrm{undop.}}(\mathbf{q}) + \delta\chi^0(\mathbf{q}, n, T), \tag{77}$$
$$\delta\chi^0(\mathbf{q}, n, T) = \frac{2}{V} \sum_{mm'\mathbf{k}} \frac{\delta f_{m\mathbf{k}} - \delta f_{m'\mathbf{k}+\mathbf{q}}}{\epsilon_{m\mathbf{k}} - \epsilon_{m'\mathbf{k}+\mathbf{q}}} |\left\langle u_{m\mathbf{k}} | u_{m'\mathbf{k}+\mathbf{q}} \right\rangle|^2,$$

and then use the RPA relation $\epsilon(\mathbf{q}, n, T) = 1 - 4\pi e^2/q^2\chi^0(\mathbf{q}, n, T)$, and $\epsilon^{-1}(\mathbf{q}, n, T) \approx 1/\epsilon(\mathbf{q}, n, T)$ to obtain the inverse of the response function, as elucidated in Eq. (7) of the main text. In particular, we plot in Fig. 6 the calculations performed in the following setups:

- Top left panel: in red we plot $\epsilon^{-1}(\mathbf{q}, n, T) \approx 1/\epsilon(\mathbf{q}, n, T)$ where $\epsilon(\mathbf{q}, n, T) = 1 - 4\pi e^2/q\chi^0(\mathbf{q}, n, T)$ and where we compute $\chi^0(\mathbf{q}, n, T)$ ab-initio from DFPT in the doped setup. In green we plot Eq. 77 evaluated on the full BZ (un-reducing the grid from the IW points) summing on 4 valence bands plus 4 conduction bands, where $\chi^{0,\text{undop.}}(\mathbf{q})$ is computed via ab-initio DFPT in the undoped setup, evaluating $\epsilon_{n\mathbf{k}}, \epsilon_{m\mathbf{k}+\mathbf{q}}$ ab-initio in the doped case, using the ab-initio Fermi level to compute $\delta f_{n\mathbf{k}}, \delta f_{m\mathbf{k}+\mathbf{q}}$, and using the overlaps $\langle u_{m\mathbf{k}}|u_{m'\mathbf{k}+\mathbf{q}}\rangle$ taken from ab-initio—the only approximation for both calculation is the neglect of local fields. The procedure to evaluate Eq. 77 is the same used for the blue dashed line of Fig. (3) of the main text, with the difference that in that case we introduce local field corrections by directly computing $1/\epsilon^{-1,\text{undop.}}(\mathbf{q})$ and the band energies are taken from Wannier interpolation.

- Top central panel: same as top left panel, but with the approximation $\langle u_{m\mathbf{k}}|u_{m'\mathbf{k}+\mathbf{q}}\rangle = \delta_{mn}$.

- Top right panel: same as top central panel, excluding the 4 conduction bands from the sum.

- Bottom left panel: same as top right panel, but where instead of using $\chi^{0,\text{undop.}}(\mathbf{q})$ we use $\chi^{0,\text{undop.}}(\mathbf{q}) \approx \chi^{0,\text{undop.}}(\mathbf{0})$.

- Bottom central panel: in red we plot $\epsilon^{-1}(\mathbf{q}, n, T)$ as obtained from DFPT calculations, in green we plot the same quantity as in the bottom left panel but where instead of $\chi^{0,\text{undop.}}(\mathbf{q}) \approx \chi^{0,\text{undop.}}(\mathbf{0})$ we use $\chi^{0,\text{undop.}}(\mathbf{q}) \approx -q^2/(4\pi e^2)(1 - 1/\epsilon^{-1,\text{undop.}}(\mathbf{q}))$ where now we include local field correction by directly computing $1/\epsilon^{-1,\text{undop.}}(\mathbf{q})$ from ab-initio.

- Bottom right panel: same as bottom central panel, but where the energies are now taken from the wannierization of the undoped valence band manifold.

From Fig. 6 we can safely conclude that the by far dominant approximation is the one on the overlap matrix elements. We also notice that, given the smooth behaviour of the dielectric

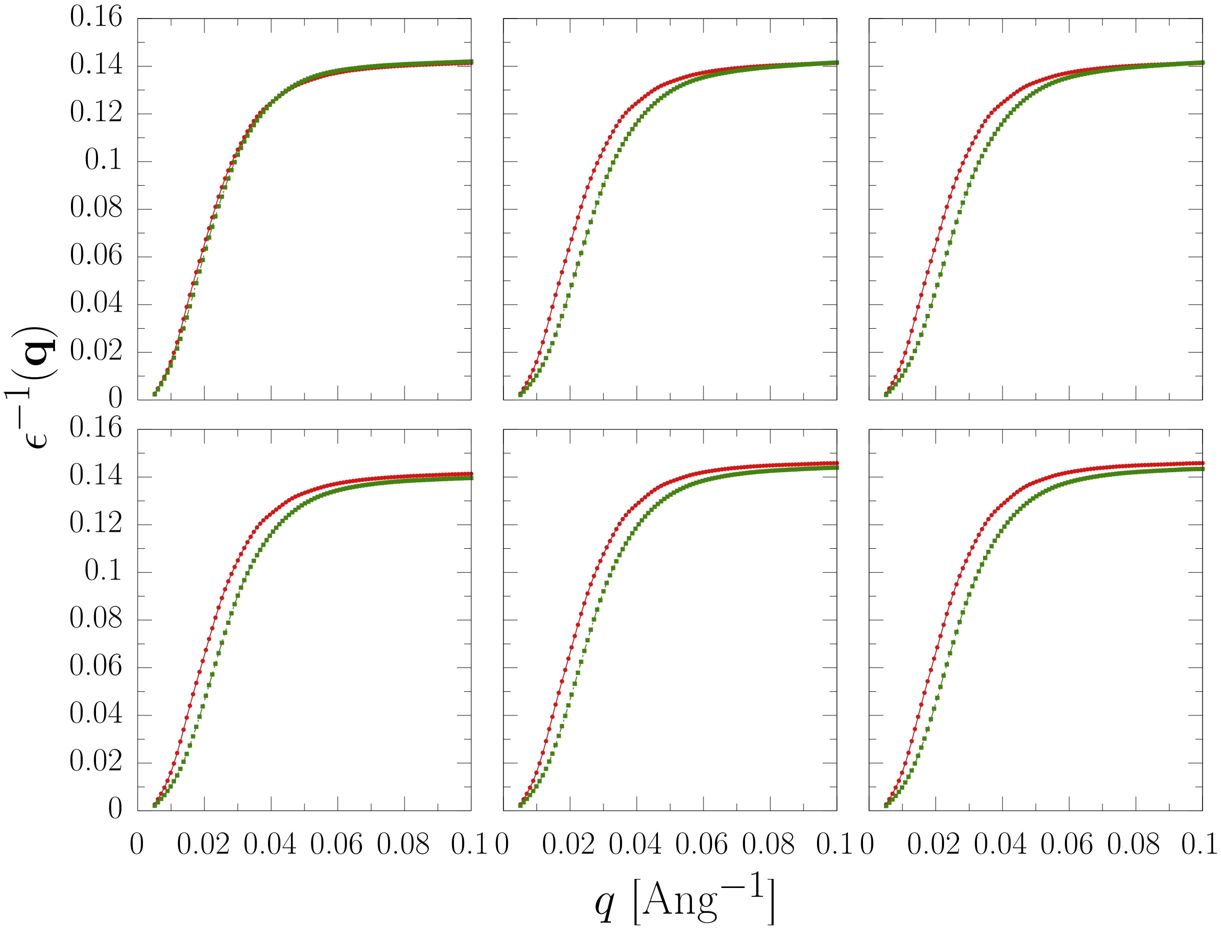


FIG. 6: *Various approximations to the response function computed with Eq. 7 of the main text.*

function, its computation can be performed on a coarse set of points, while the evaluation on a fine mesh can be obtained by a simple polynomial interpolation.

## UNSCREENED CHARGE DENSITY IN THE UNDOPED CASE

In this section we want to verify our implementation of the unscreening of the charge density change in presence of $\delta\rho^{\text{ext}}_{s,\alpha}$. In particular, we compare in Fig. 7 the charge density change by including or not including the macroscopic part of the total potential at $\mathbf{G} = 0$. In both cases, the results agree with theoretical expectations.

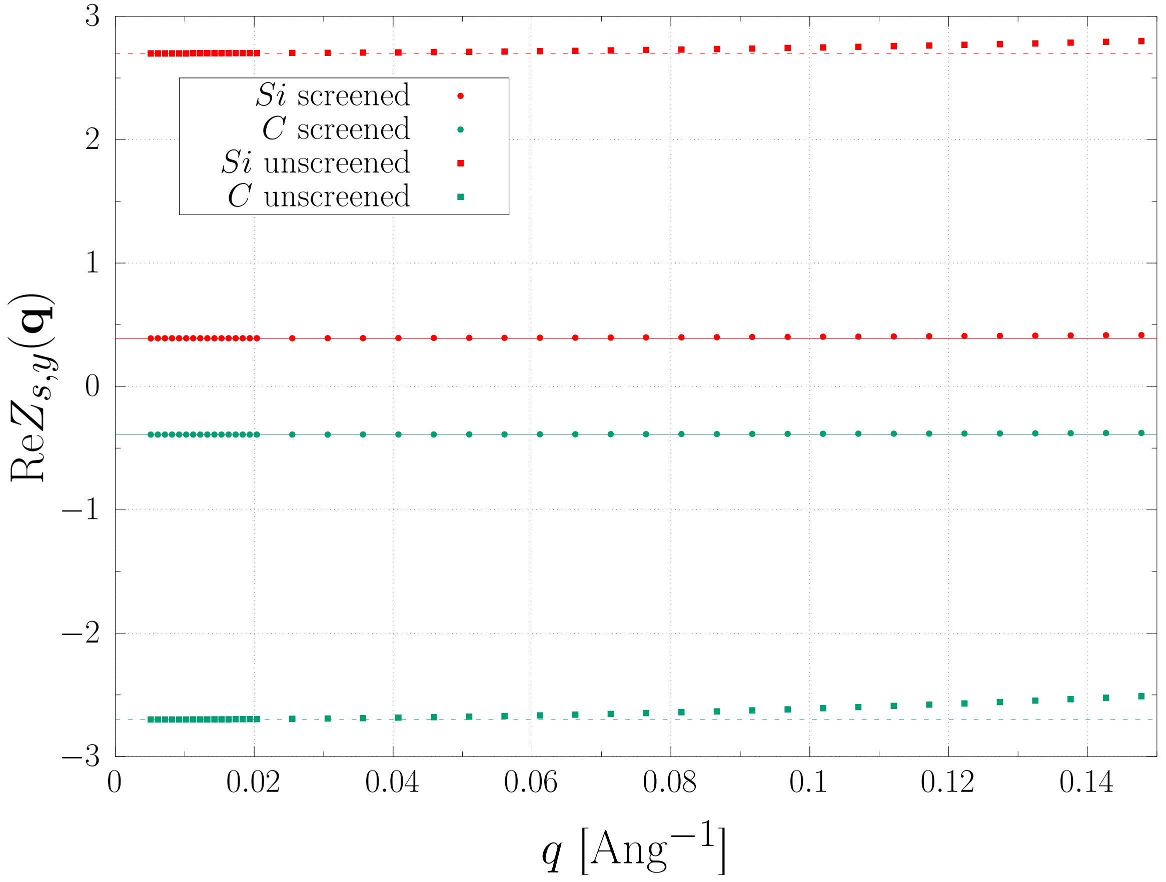


FIG. 7: *Real part of the effective charge tensor for the undoped and doped cases, as a function of $q$ along the line $\mathbf{q} = (q/\sqrt{2}, q/\sqrt{2}, 0)$, for the Si atom. The continuous and dashed lines are drawn using the expressions of Eqs. (5) and (6) of the main text using $\epsilon^\infty = 6.9179$ and $\epsilon^\infty = 1$.*

[1] M. Stengel, Phys. Rev. B **88**, 174106 (2013).

[2] S. Baroni, S. de Gironcoli, A. Dal Corso, and P. Giannozzi, Rev. Mod. Phys. **73**, 515 (2001).

[3] R. Senga, K. Suenaga, P. Barone, S. Morishita, F. Mauri, and T. Pichler, Nature **573**, 247 (2019).

[4] R. M. Pick, M. H. Cohen, and R. M. Martin, Phys. Rev. B **1**, 910 (1970).

[5] P. Ghosez, X. Gonze, and R. W. Godby, Phys. Rev. B **56**, 12811 (1997).

[6] P. Vogl, Phys. Rev. B **13**, 694 (1976).

[7] G. Brunin, H. P. C. Miranda, M. Giantomassi, M. Royo, M. Stengel, M. J. Verstraete, X. Gonze, G.-M. Rignanese, and G. Hautier, Phys. Rev. Lett. **125**, 136601 (2020).

[8] P. Giannozzi, O. Baseggio, P. Bonfà, D. Brunato, R. Car, I. Carnimeo, C. Cavazzoni, S. de Gironcoli, P. Delugas, F. Ferrari Ruffino, A. Ferretti, N. Marzari, I. Timrov, A. Urru, and S. Baroni, The Journal of Chemical Physics **152**, 154105 (2020), https://doi.org/10.1063/5.0005082.

[9] J. P. Perdew, K. Burke, and M. Ernzerhof, Phys. Rev. Lett. **77**, 3865 (1996).

[10] S. Poncé, F. Macheda, E. R. Margine, N. Marzari, N. Bonini, and F. Giustino, Phys. Rev. Research **3**, 043022 (2021).

[11] L. Binci, P. Barone, and F. Mauri, Phys. Rev. B **103**, 134304 (2021).

[12] S. Poncé, E. Margine, C. Verdi, and F. Giustino, Computer Physics Communications **209**, 116 (2016).

[13] T. Sohier, M. Calandra, and F. Mauri, Phys. Rev. B **91**, 165428 (2015).

[14] M. Royo and M. Stengel, Phys. Rev. X **9**, 021050 (2019).

[15] J. Hong and D. Vanderbilt, Phys. Rev. B **84**, 180101 (2011).
